# Supplementary material for: 28 -- 40 GHz variability and polarimetry of bright compact sources in the QUIJOTE cosmological fields
Source: arXiv:2102.04520 ancillary file (2021-02-08)
Supplement: Supplementary file 1 [file appendix_r3-compressed.pdf]

APPENDIX A: MAP- AND  $uv$ -PLANE RESIDUALS

Here we show map- and  $uv$ -plane residuals for each 28 – 40 GHz VLA observation of each source after subtracting the compact core assuming a point source model. See the caption of the first figure in each subsection for more detail.

## A1 Sources with residuals &lt; 1% of the point source flux density

In the cases in this subsection, the map and  $uv$ -plane residuals were < 1% of the point source flux density at the central frequency (indicated by the horizontal dashed lines), and so we did not perform any additional self-calibration.

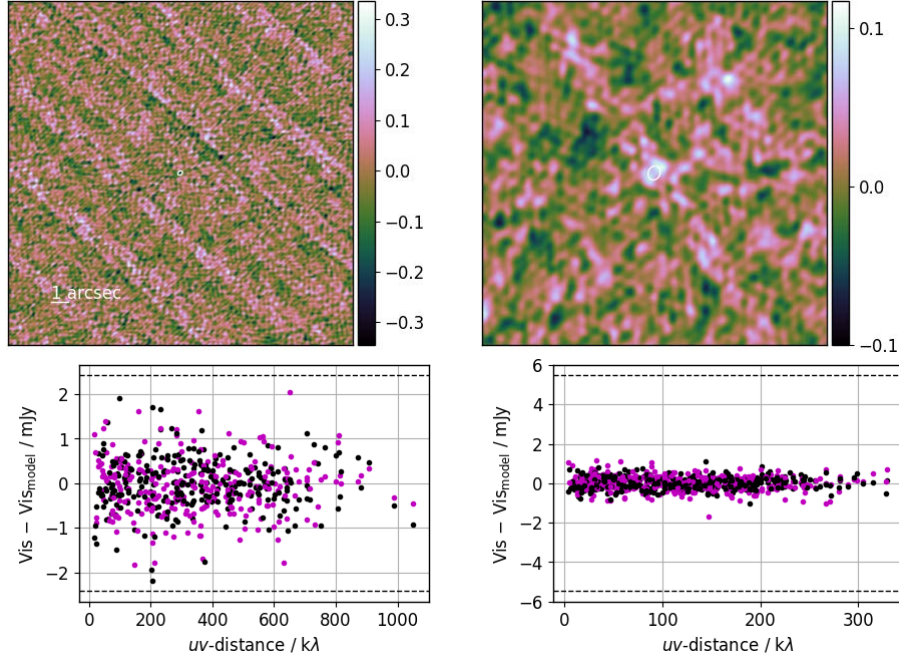

**Figure A1.** Residuals after subtracting the point-source model in the map-plane (top) and  $uv$ -plane (bottom), for PCCS1 030 G107.00-50.62. The first observation is on the left in each row and the second observation on the right. The colour-scale for the maps is in mJy/beam; the angular scale is indicated with the horizontal line on the left-hand map and the 50% contour of the synthesised beam is shown at the position of the subtracted point source on each map. The field of view is the same in the two maps. The maps have not been cleaned. In the  $uv$ -plane plots, the residual visibility data have been averaged over frequency (28 – 40 GHz) and time to leave one point per baseline; magenta and black points are real and imaginary components respectively. The horizontal black dashed lines indicate 1% of the point source flux density at the central frequency at each epoch.

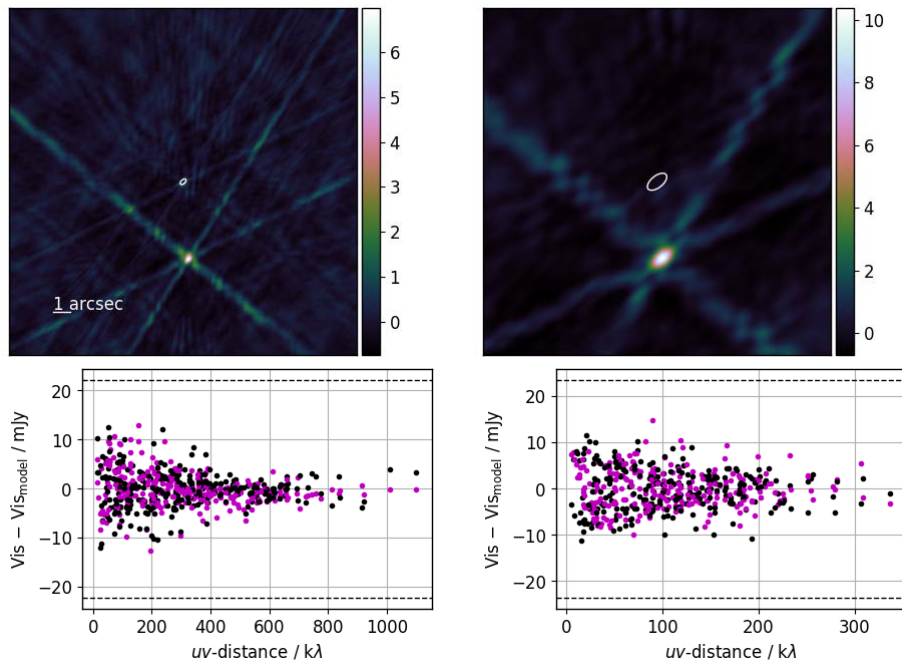

**Figure A2.** Residual plots for PCCS1 030 G131.84-60.98; see caption for Fig. A1 for more detail.

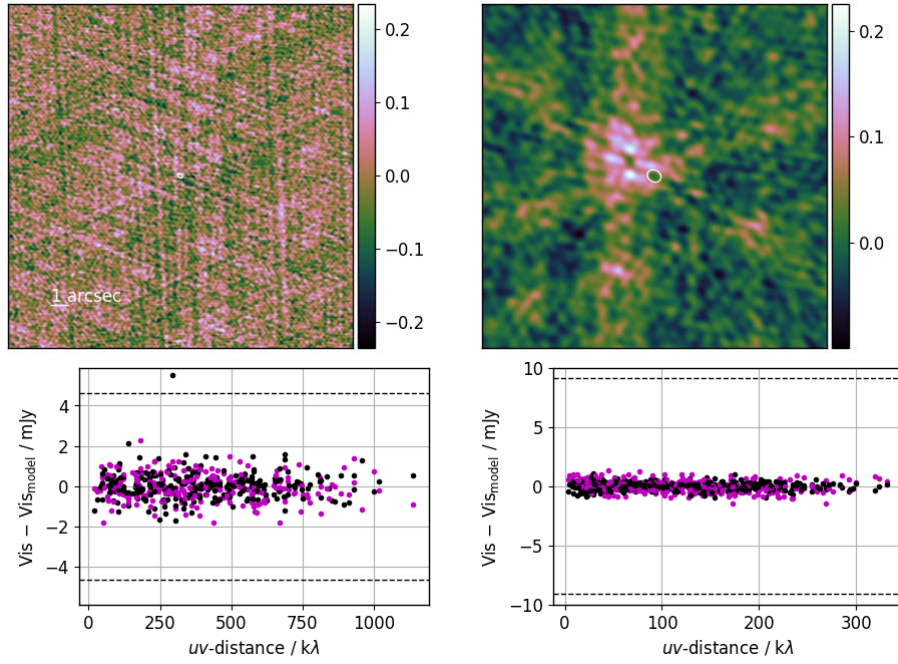

**Figure A3.** Residual plots for PCCS1 030 G129.09-13.46; see caption for Fig. A1 for more detail.

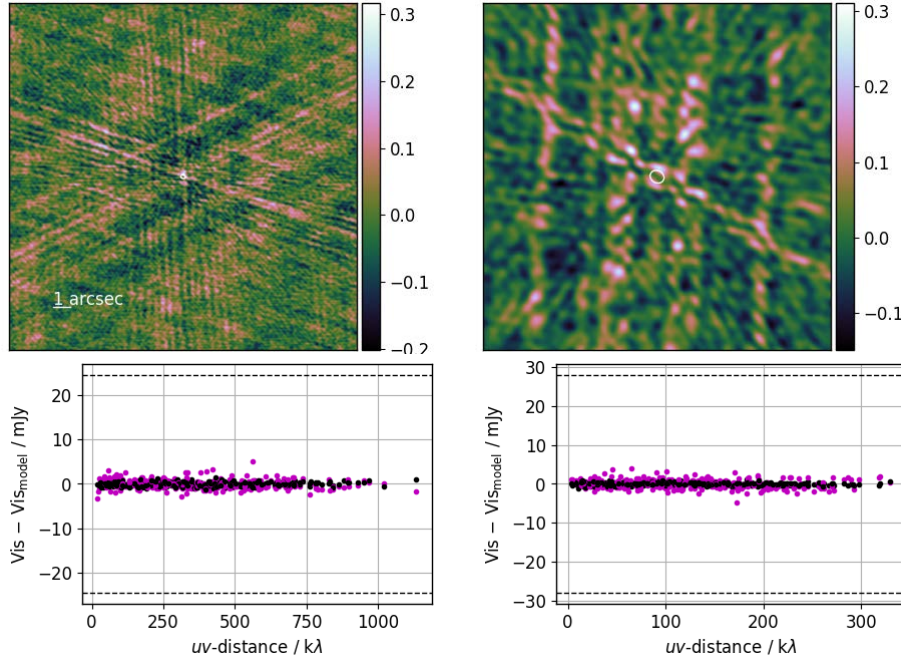

**Figure A4.** Residual plots for PCCS1 030 G130.78-14.31; see caption for Fig. A1 for more detail.

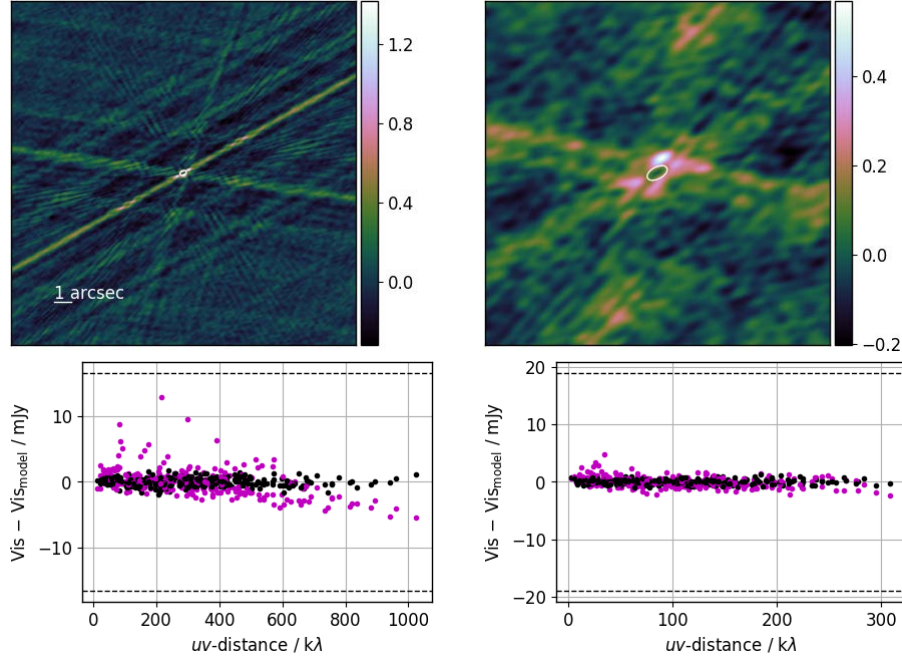

**Figure A5.** Residual plots for PCCS1 030 G141.09-38.56; see caption for Fig. A1 for more detail.

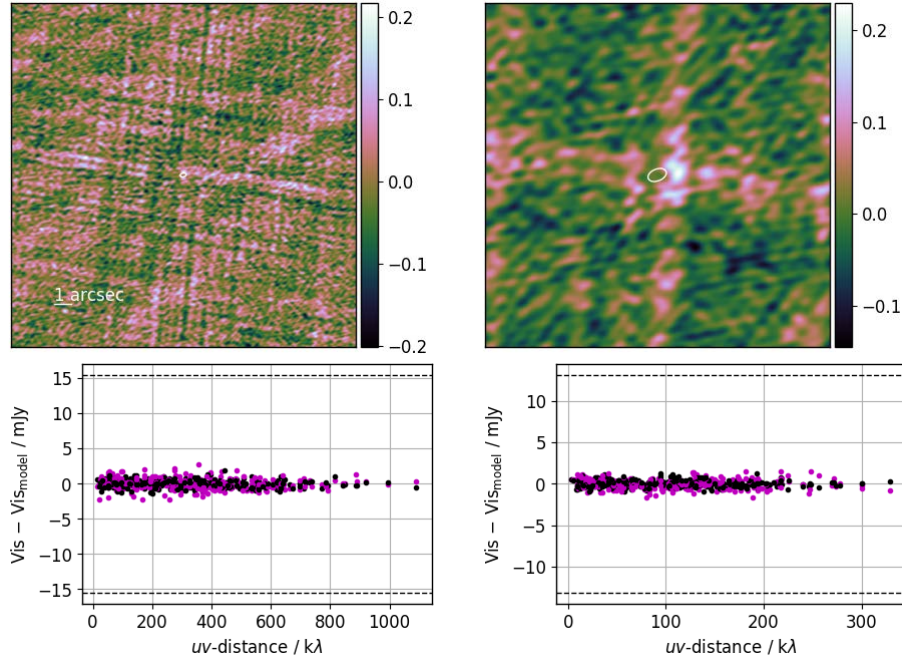

**Figure A6.** Residual plots for PCCS1 030 G140.56-28.12; see caption for Fig. A1 for more detail.

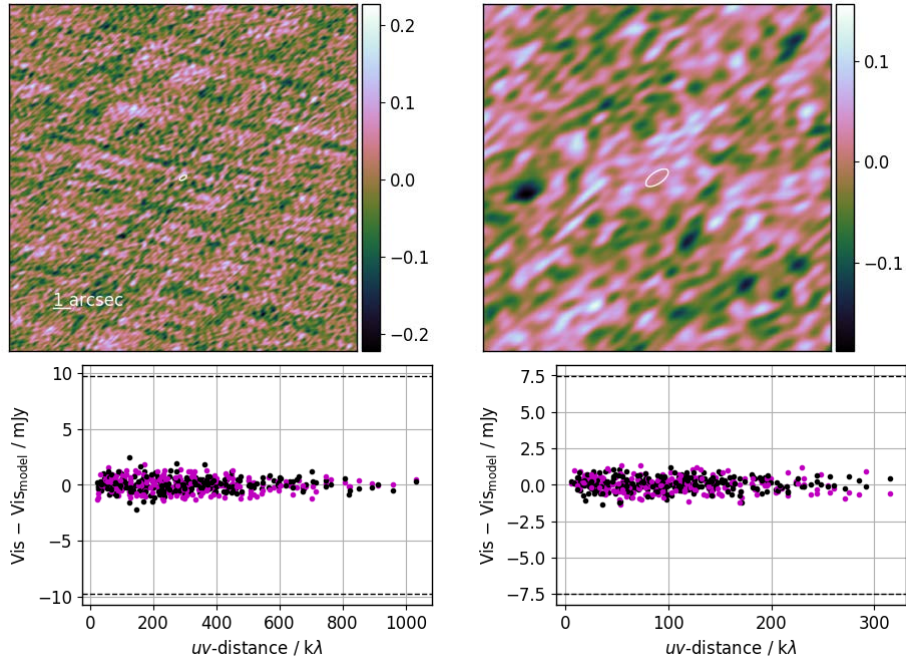

**Figure A7.** Residual plots for PCCS1 030 G152.57-47.29; see caption for Fig. A1 for more detail.

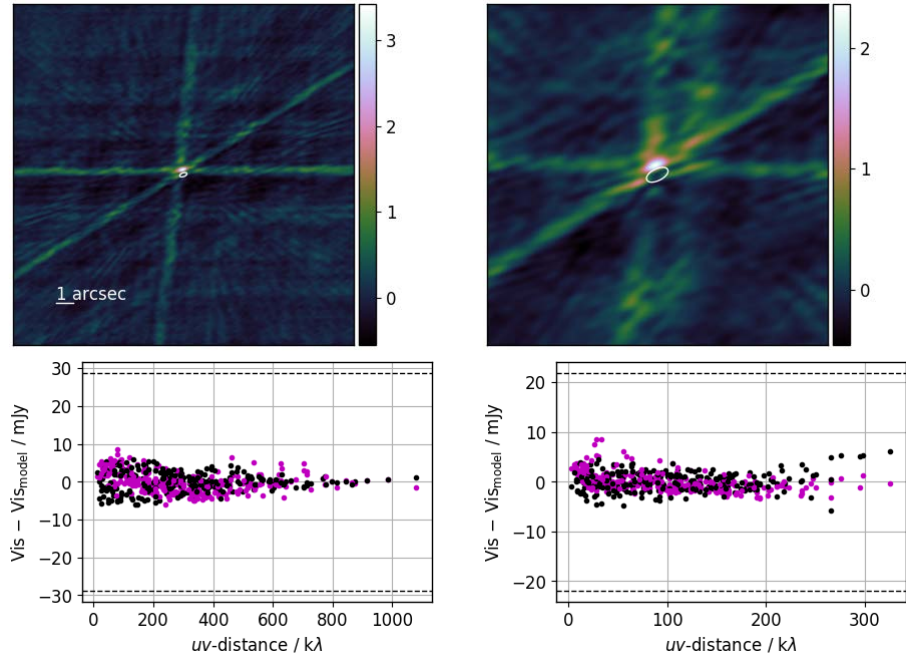

**Figure A8.** Residual plots for PCCS1 030 G149.50-28.53; see caption for Fig. A1 for more detail.

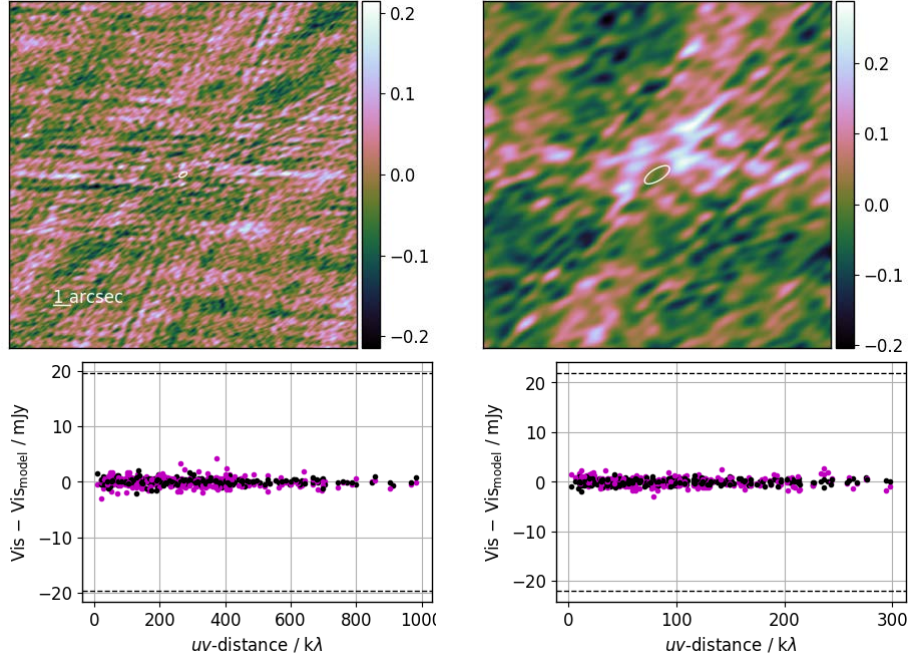

**Figure A9.** Residual plots for PCCS1 030 G156.86-39.13; see caption for Fig. A1 for more detail.

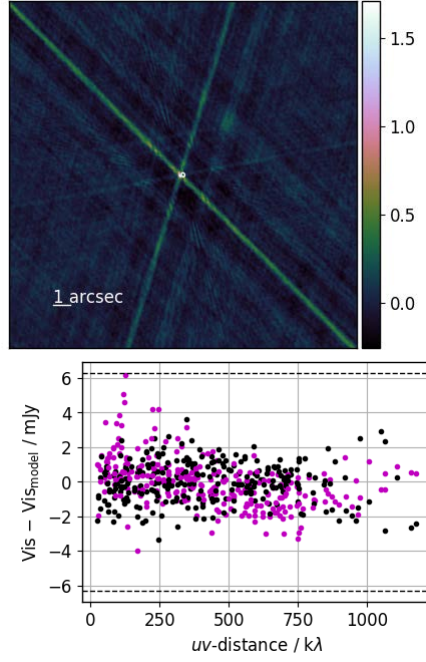

**Figure A10.** Residual plots for PCCS1 030 G178.26+33.40; see caption for Fig. A1 for more detail. In this case there is only one observing epoch.

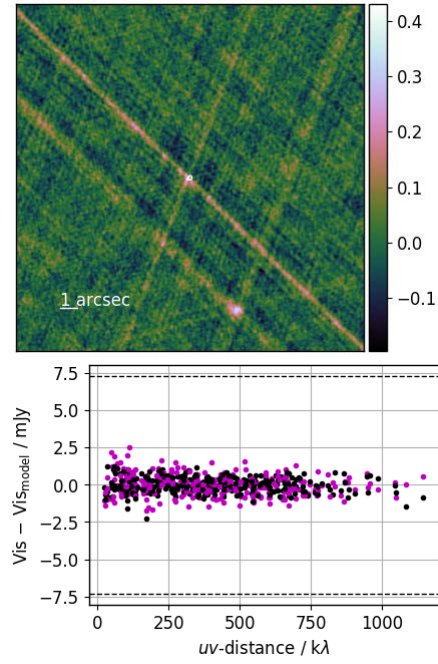

**Figure A11.** Residual plots for PCCS1 030 G200.04+31.88; see caption for Fig. A1 for more detail. In this case there is only one observing epoch.

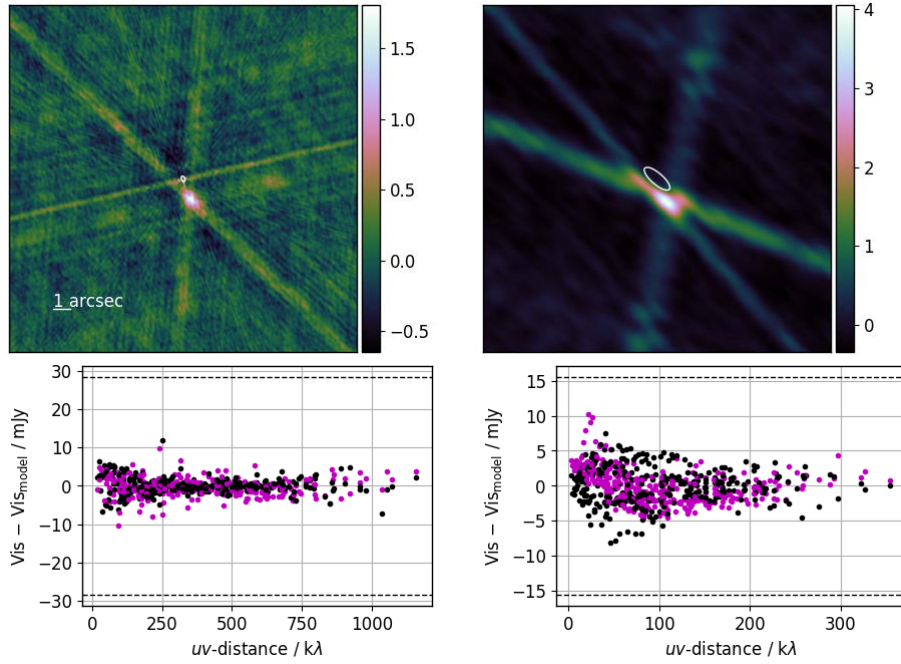

**Figure A12.** Residual plots for PCCS1 030 G143.53+34.42; see caption for Fig. A1 for more detail.

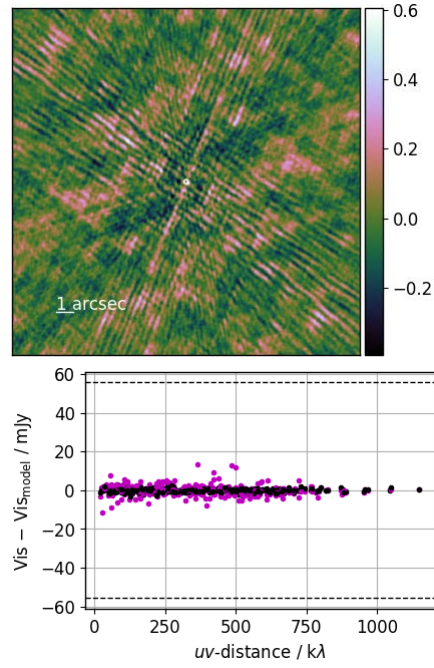

**Figure A13.** Residual plots for PCCS1 030 G206.82+35.81; see caption for Fig. A1 for more detail. In this case there is only one observing epoch.

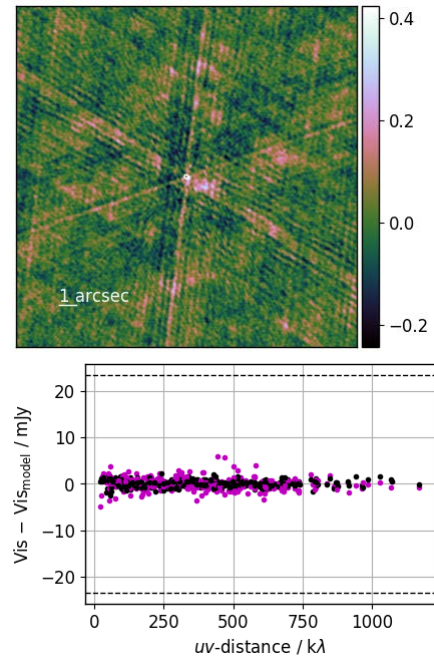

**Figure A14.** Residual plots for PCCS1 030 G175.72+44.81; see caption for Fig. A1 for more detail. In this case there is only one observing epoch.

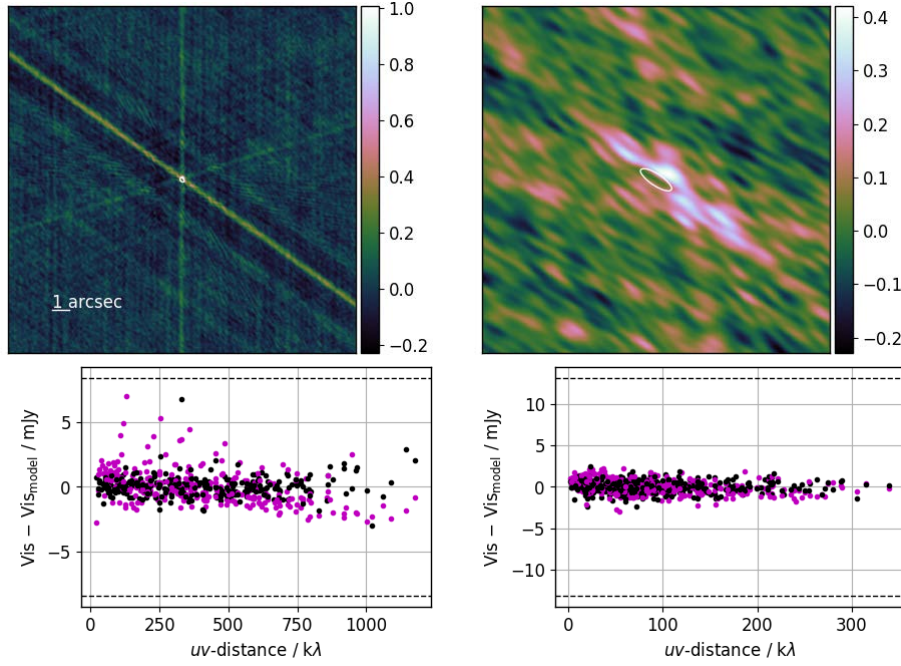

**Figure A15.** Residual plots for PCCS1 030 G152.23+41.00; see caption for Fig. A1 for more detail.

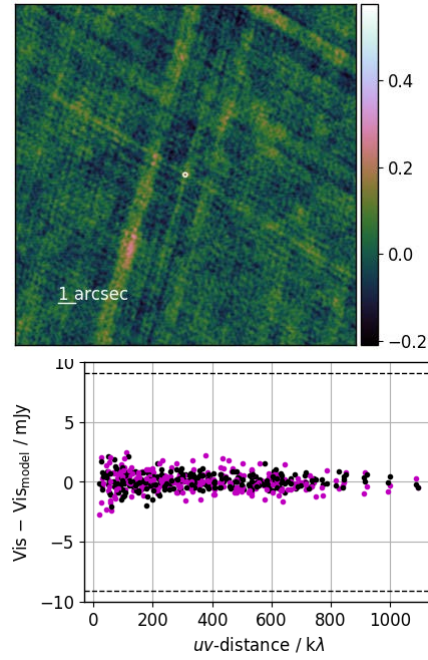

**Figure A16.** Residual plots for PCCS1 030 G198.82+44.43; see caption for Fig. A1 for more detail. In this case there is only one observing epoch.

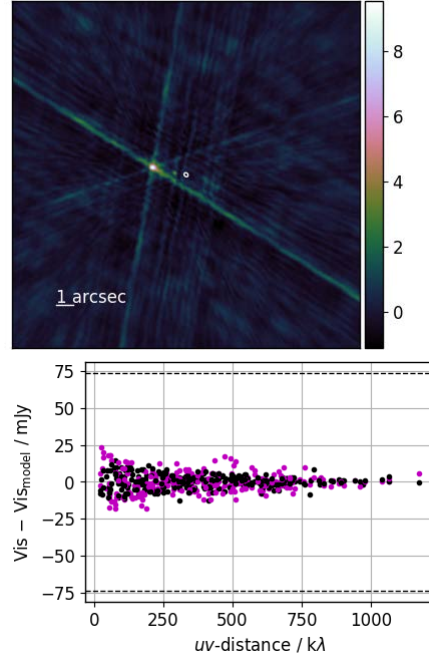

**Figure A17.** Residual plots for PCCS1 030 G183.71+46.17; see caption for Fig. A1 for more detail. In this case there is only one observing epoch.

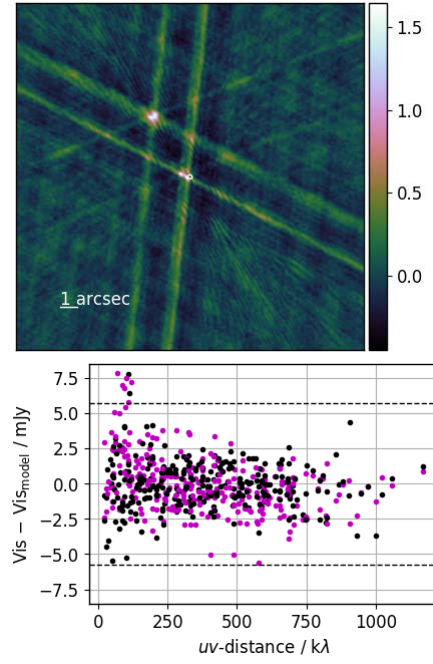

**Figure A18.** Residual plots for PCCS1 030 G181.02+50.29; see caption for Fig. A1 for more detail. In this case there is only one observing epoch.

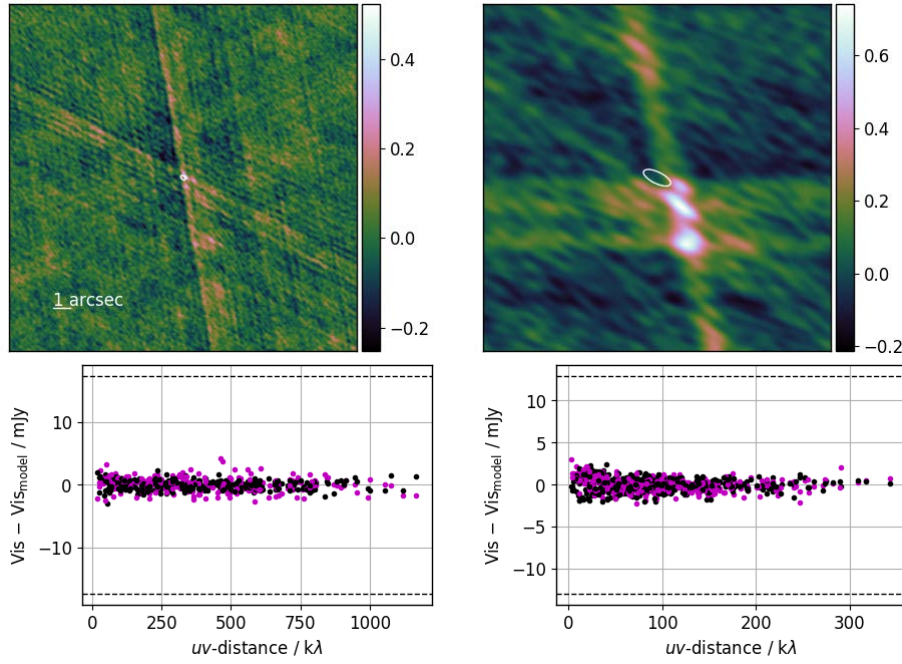

**Figure A19.** Residual plots for PCCS1 030 G145.78+43.13; see caption for Fig. A1 for more detail.

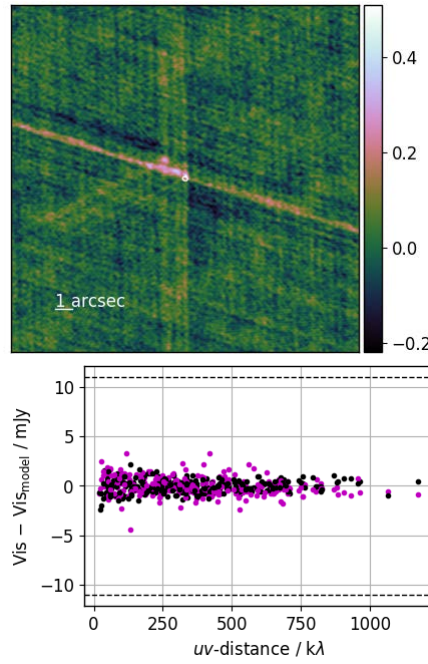

**Figure A20.** Residual plots for PCCS1 030 G177.37+58.35; see caption for Fig. A1 for more detail. In this case there is only one observing epoch.

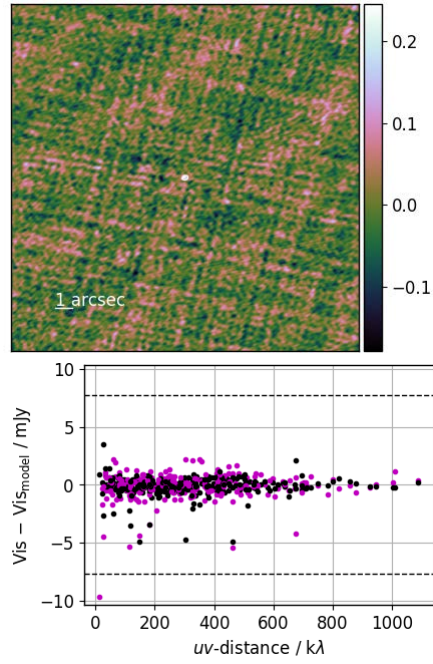

**Figure A21.** Residual plots for PCCS1 030 G211.56+60.99; see caption for Fig. A1 for more detail. In this case there is only one observing epoch.

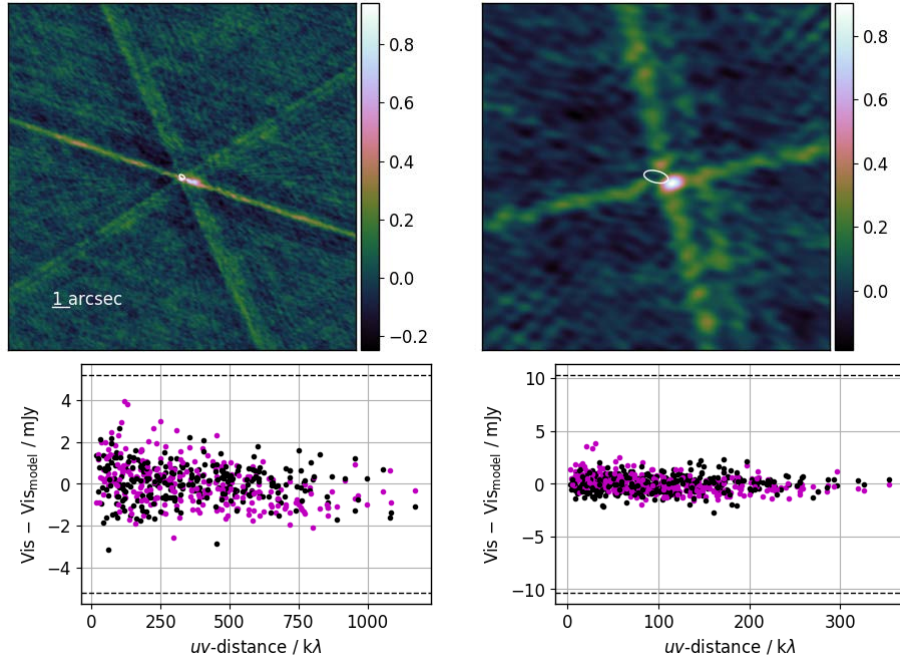

**Figure A22.** Residual plots for PCCS1 030 G135.47+42.26; see caption for Fig. A1 for more detail.

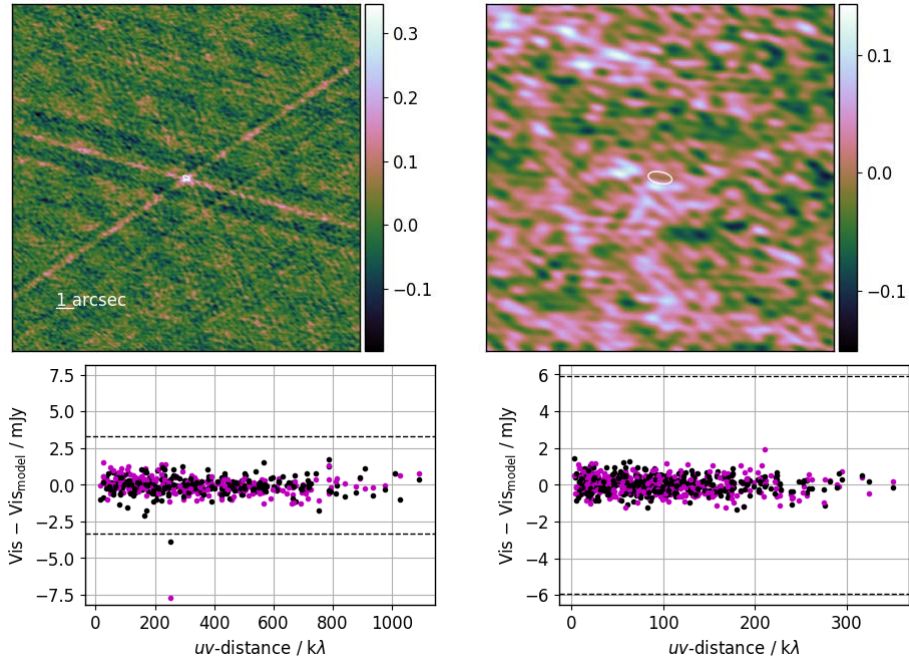

**Figure A23.** Residual plots for PCCS1 030 G135.91+43.92; see caption for Fig. A1 for more detail.

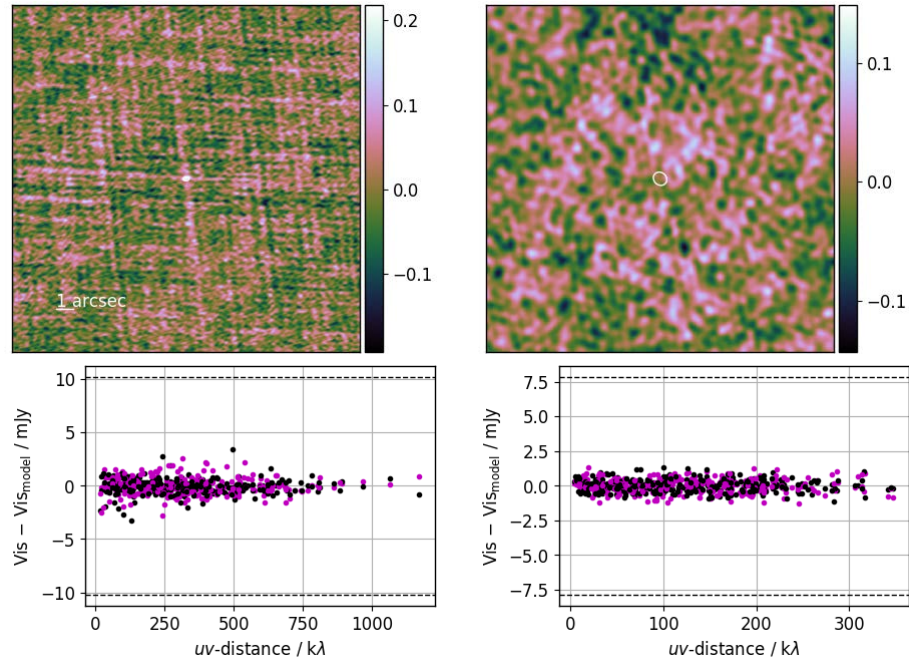

**Figure A24.** Residual plots for PCCS1 030 G174.43+69.81; see caption for Fig. A1 for more detail.

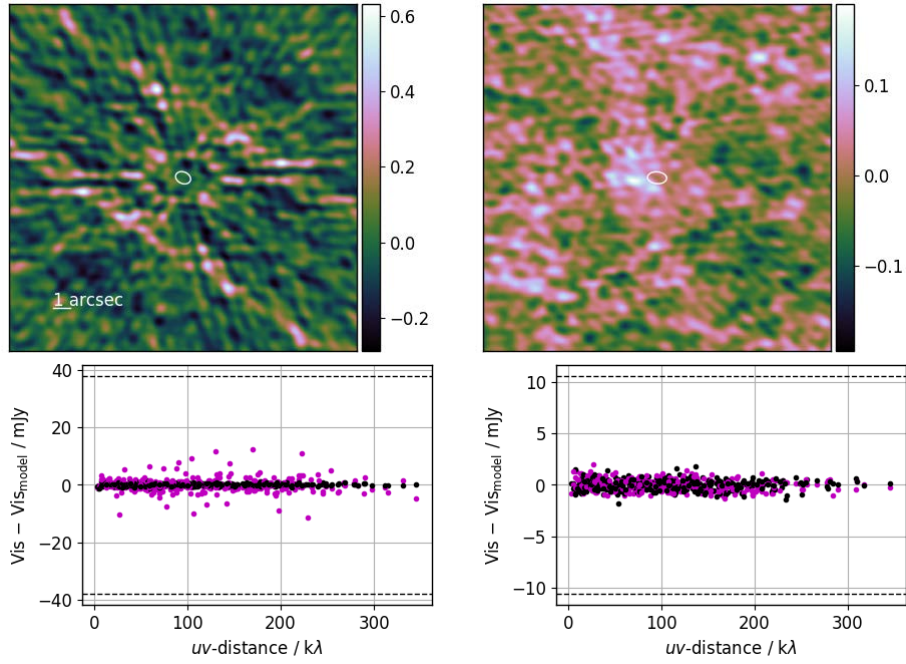

**Figure A25.** Residual plots for PCCS1 030 G098.27+58.31; see caption for Fig. A1 for more detail.

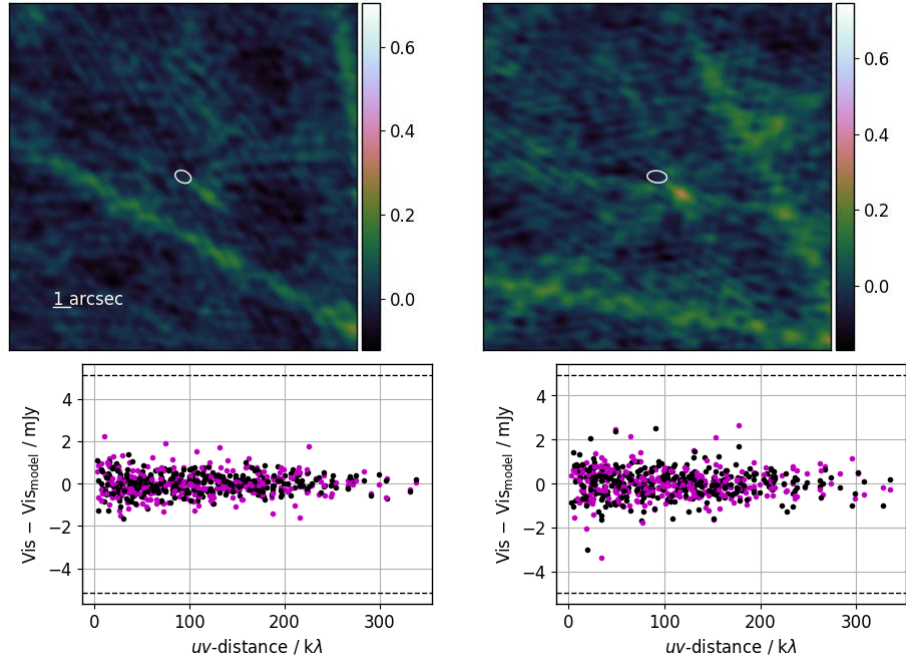

**Figure A26.** Residual plots for PCCS1 030 G105.20+49.72; see caption for Fig. A1 for more detail.

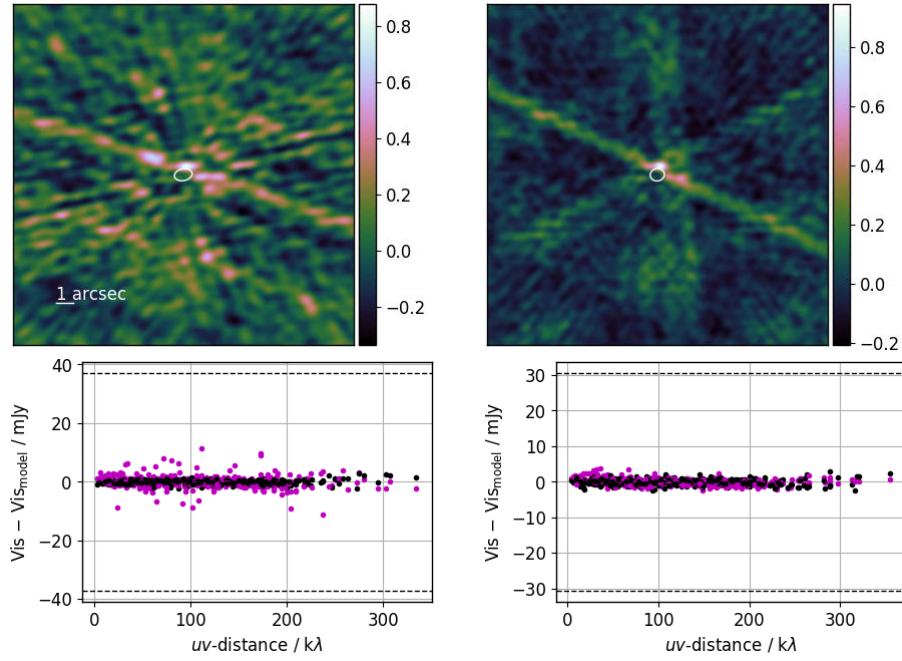

**Figure A27.** Residual plots for PCCS1 030 G055.14+46.37; see caption for Fig. A1 for more detail.

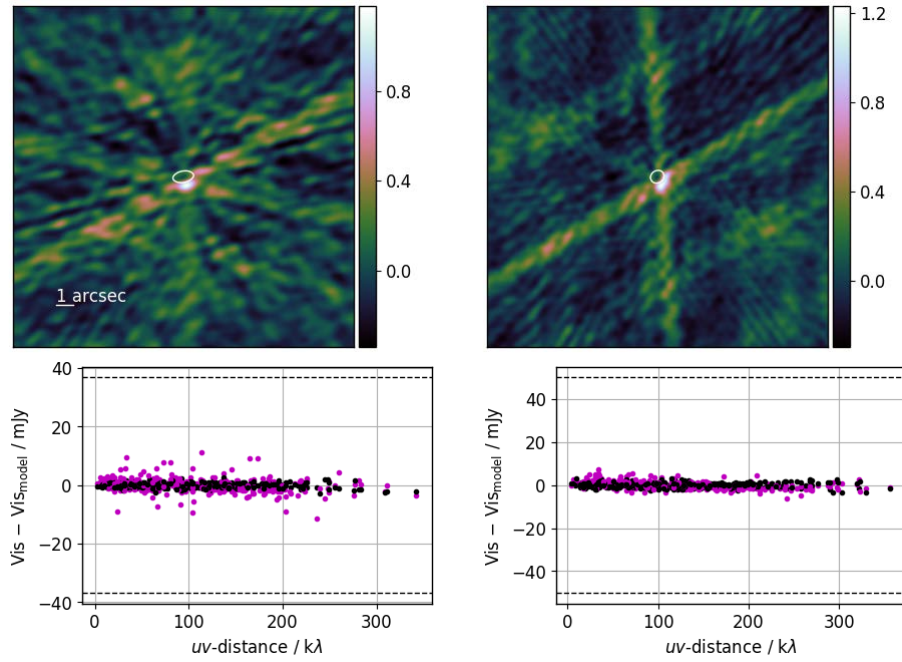

**Figure A28.** Residual plots for PCCS1 030 G061.07+42.34; see caption for Fig. A1 for more detail.

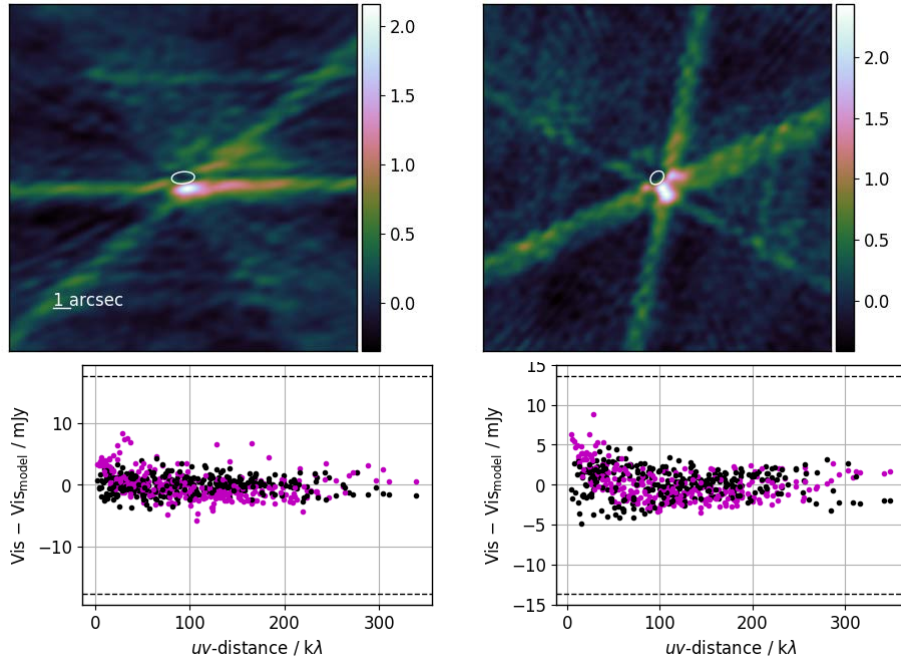

**Figure A29.** Residual plots for PCCS1 030 G086.64+40.35; see caption for Fig. A1 for more detail.

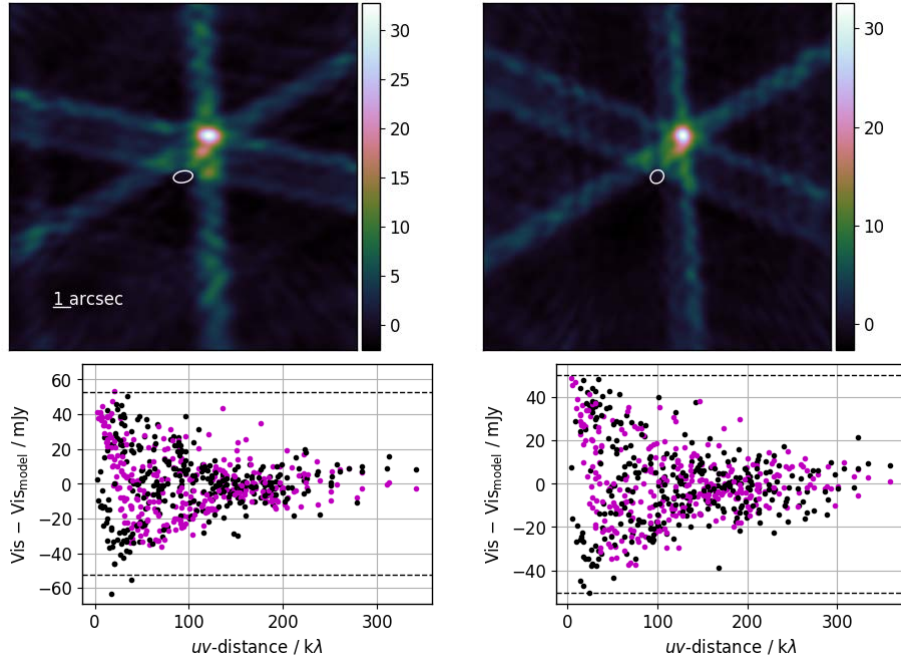

**Figure A30.** Residual plots for PCCS1 030 G063.46+40.96; see caption for Fig. A1 for more detail.

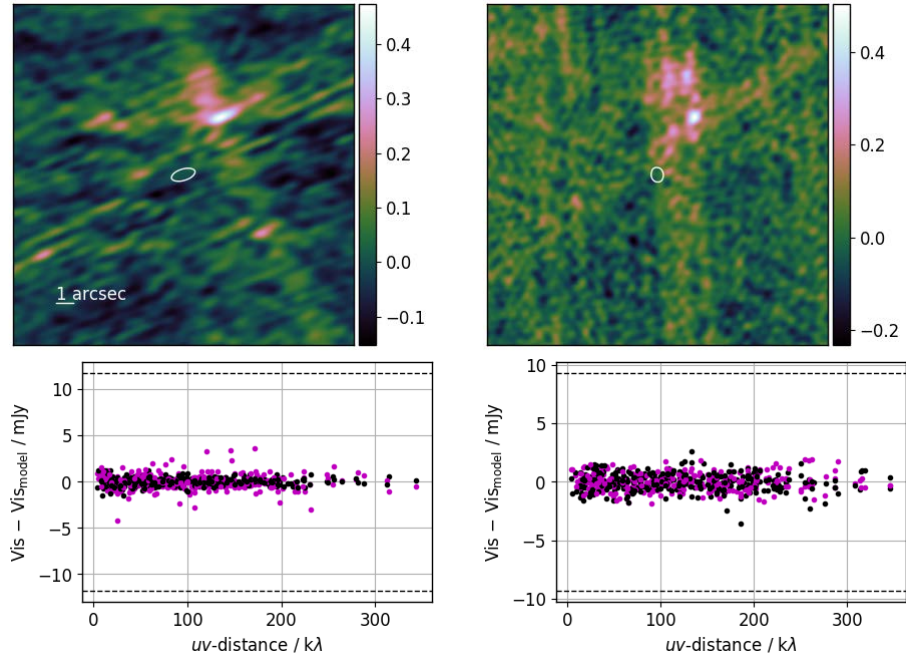

**Figure A31.** Residual plots for PCCS1 030 G071.46+33.28; see caption for Fig. A1 for more detail.

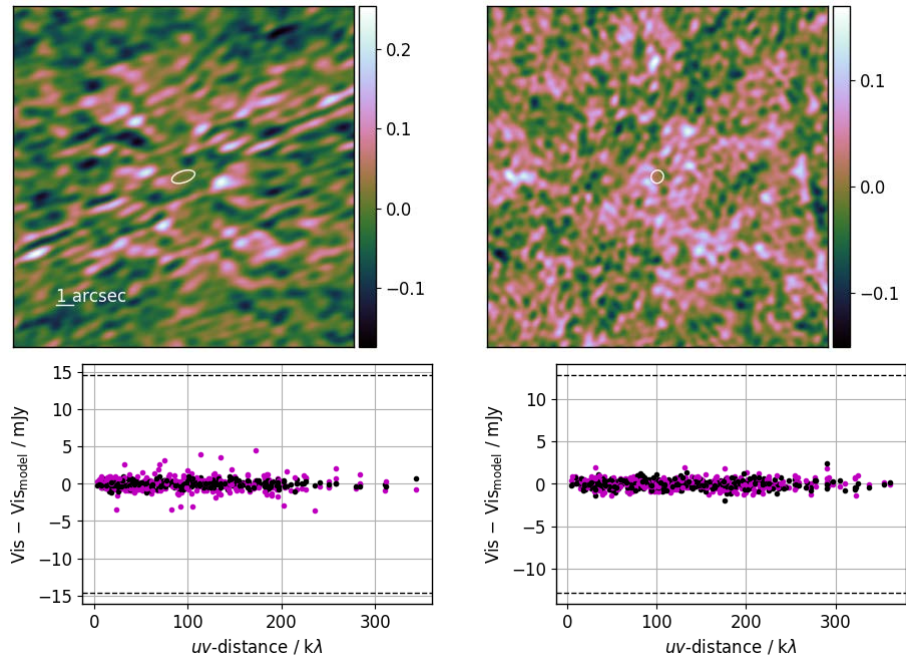

**Figure A32.** Residual plots for PCCS1 030 G064.03+31.01; see caption for Fig. A1 for more detail.

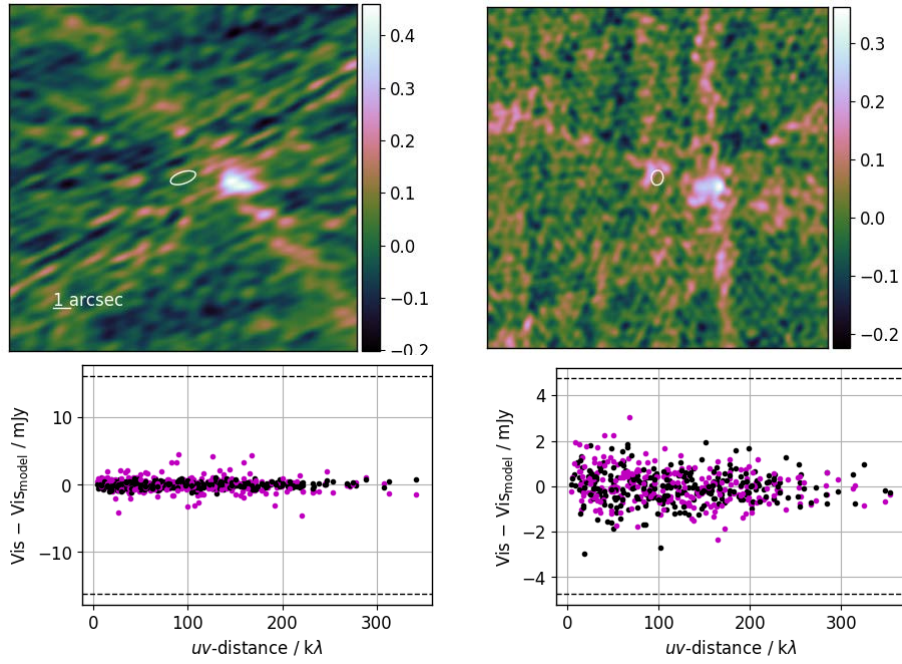

**Figure A33.** Residual plots for PCCS1 030 G079.56+31.72; see caption for Fig. A1 for more detail.

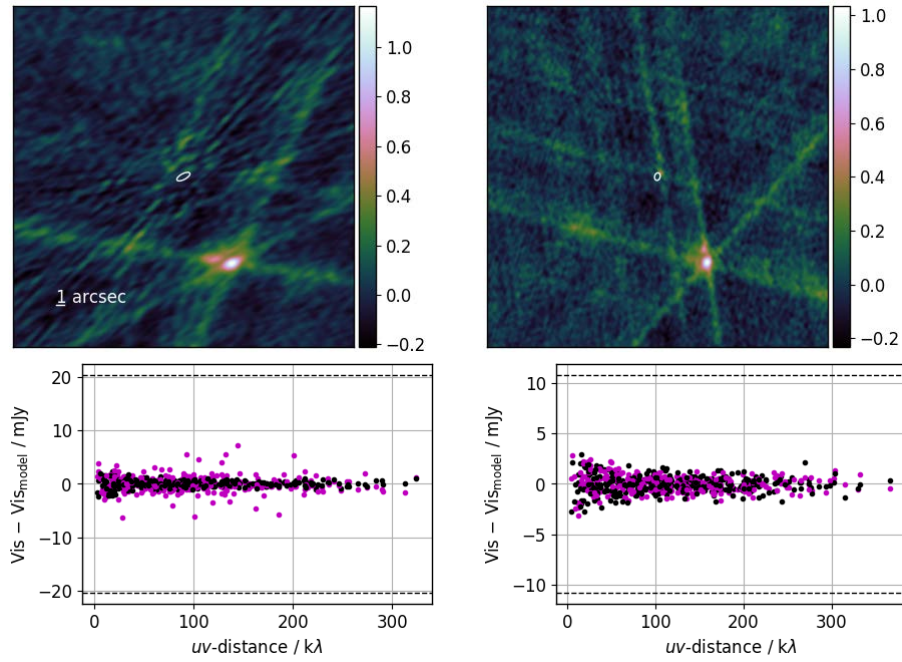

**Figure A34.** Residual plots for PCCS1 030 G097.50+25.03; see caption for Fig. A1 for more detail.

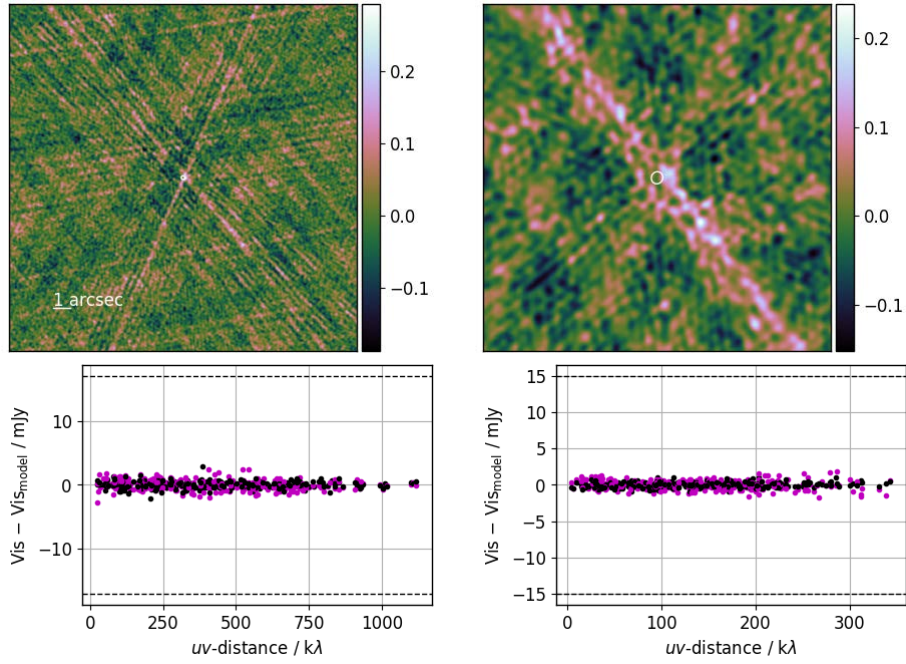

**Figure A35.** Residual plots for PCCS1 030 G090.09-25.64; see caption for Fig. A1 for more detail.

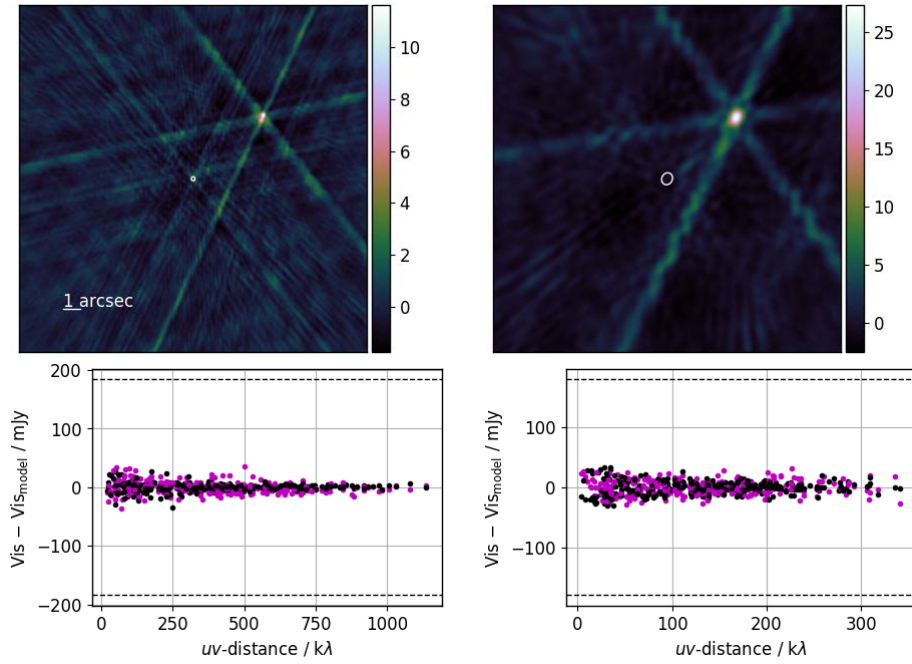

**Figure A36.** Residual plots for PCCS1 030 G086.10-38.18; see caption for Fig. A1 for more detail.

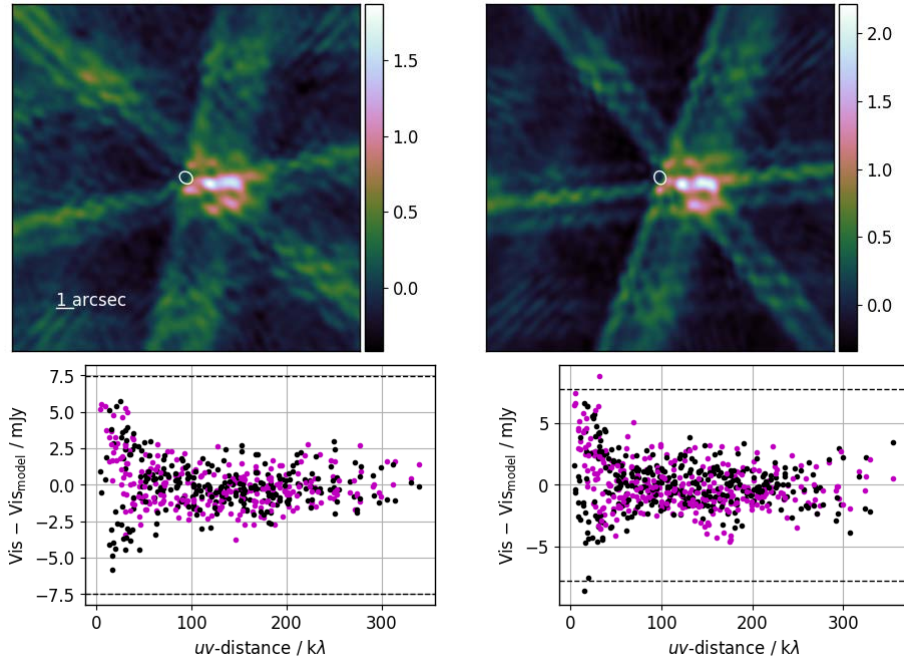

**Figure A37.** Residual plots for PCCS1 030 G108.97-09.47; see caption for Fig. A1 for more detail.

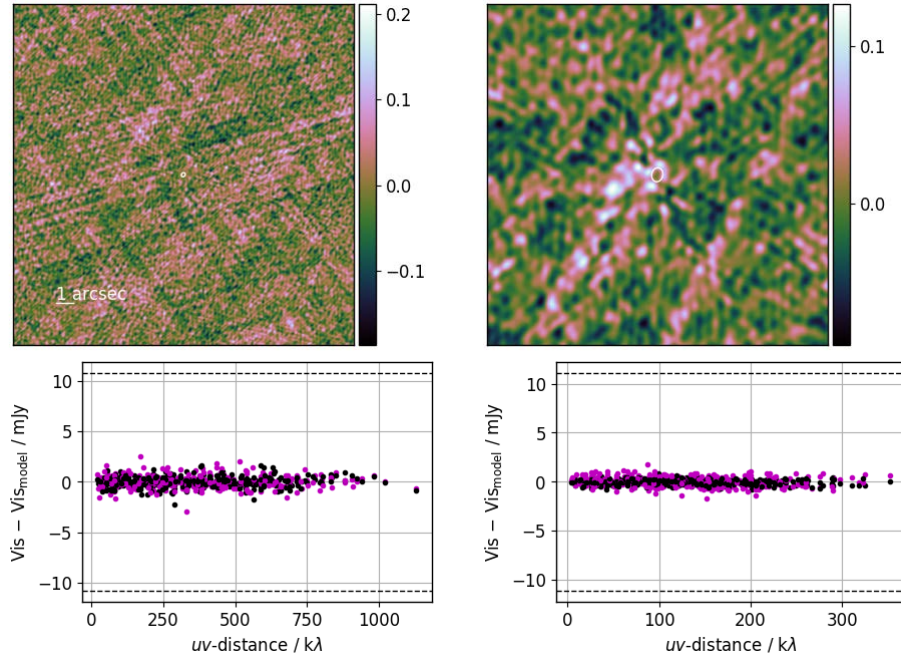

**Figure A38.** Residual plots for PCCS1 030 G091.12-47.97; see caption for Fig. A1 for more detail.

**A2 Sources with residuals  $> 1\%$  of the point source flux density**

In these cases, the non-core flux density was  $> 1\%$  of the point source flux density at the central frequency, and we performed an extra self-calibration step as follows. For each source we made a combined, core-subtracted map from both observations (top left) which we used to create a  $uv$ -plane model (bottom left) which was added to the core point source model to iteratively improve the amplitude solution for the core. We subtract the combined model (+ variable point-source component) from each individual observation and show the resulting residual maps (top middle and right) and  $uv$ -plane residuals (bottom middle and right). In some cases we performed the calibration using particular baseline lengths; these are indicated by black vertical lines and the subtracted maps are made by restricting to this  $uv$ -range. Where observations were performed with different VLA array configurations, we used the common  $uv$ -range to perform the self-calibration so we could be sure to eliminate any bias due to resolution.

In some cases, particularly when the observations were separated by over 2 years (PCCS1 030 G073.40+41.88, PCCS1 030 G100.68+36.62, PCCS1 030 G100.13+29.16, PCCS1 030 G085.73+26.11, PCCS1 030 G077.23+23.50), we found the extended structure also seemed to vary between observations (much less significantly than the core). It would be difficult for these differences to be produced by resolution differences between different array configurations because we have self-calibrated both observations together to produce a combined model spanning the  $uv$ -coverage of both observations. In these cases we also performed the same self-calibration procedure on each individual observation. The difference between the individual and combined self-calibrated amplitude solutions was much less than the overall calibration error in all cases except for PCCS1 030 G077.23+23.50, which has a particularly significant, variable extended structure. The bright feature seen on the map appears to be a superposition of the ‘K1’ and ‘K2’ knot features at  $\approx 0.73$  and  $\approx 1.1$  arcsec away from the core respectively, identified by [Papageorgiou et al. \(2006\)](#). [Koyama et al. \(2013\)](#) note that the knots are strongly interacting with the ambient medium and show a significant change in structure of the K1 knot between 1998 and 2001, so it is plausible for our observations taken in 2016 and 2018 also to show a structural difference. In this case we display the combined, self-calibrated maps but take the individual amplitude solutions as our fiducial result, adding the difference between the combined self-calibrated amplitude solution and individually self-calibrated amplitude solution as an extra calibration error.

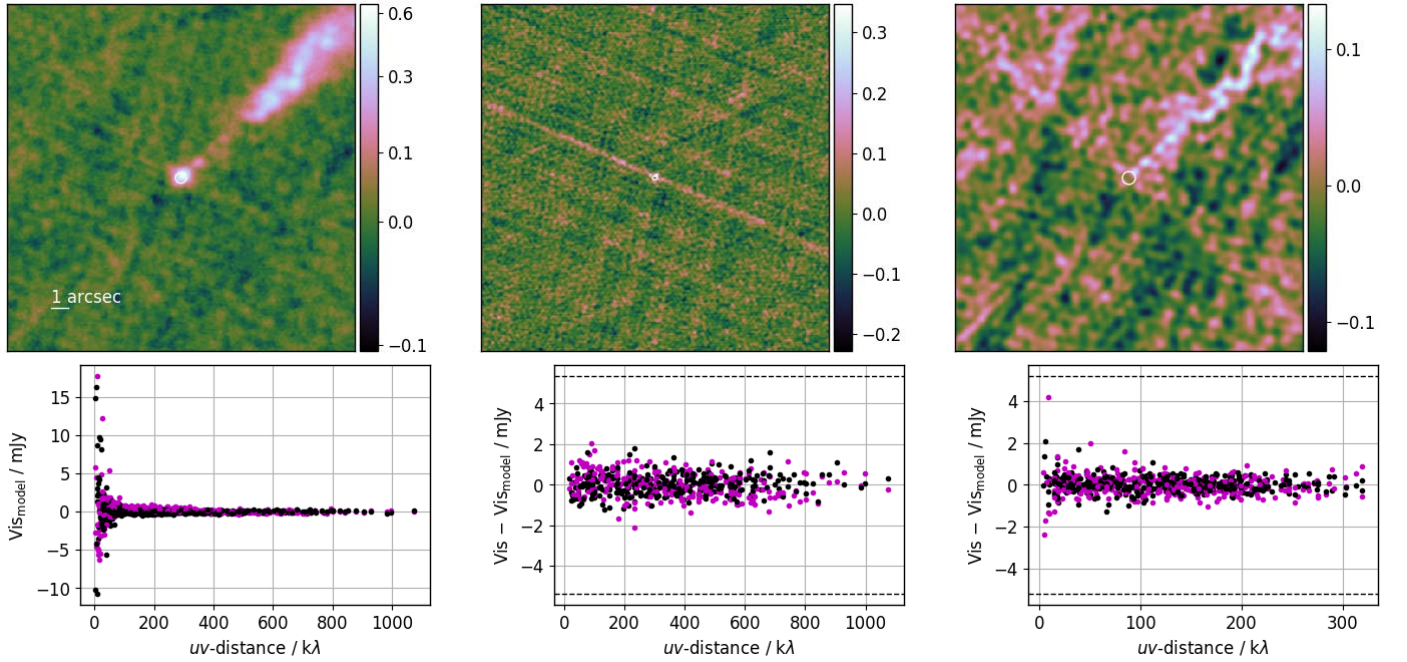

**Figure A39.** Self-calibrated map of the non-core flux density and corresponding  $uv$ -plane model (left-hand column), and residual plots for each observing epoch (centre and right-hand columns) in the map- and  $uv$ -plane, where both the point-source and non-core flux density models have been subtracted, for PCCS1 030 G124.55-32.50. The non-core flux density model is self-calibrated using both observations spanning the full  $uv$ -range of the different VLA configurations. The full model extends to a larger field of view but is truncated here to show the most significant part. As in Fig. A1, the colour-scale for the maps is in mJy/beam; the angular scale is indicated with the horizontal line on the left-hand map and the 50% contour of the synthesised beam is shown at the position of the subtracted point source on each map. The field of view is the same in the three maps. The residual maps have not been cleaned. In the  $uv$ -plane plots, the residual visibility data have been averaged over frequency (28 – 40 GHz) and time to leave one point per baseline; magenta and black points are real and imaginary components respectively. The horizontal black dashed lines on the residual  $uv$ -plane plots indicate 1% of the point source flux density at the central frequency at each epoch.

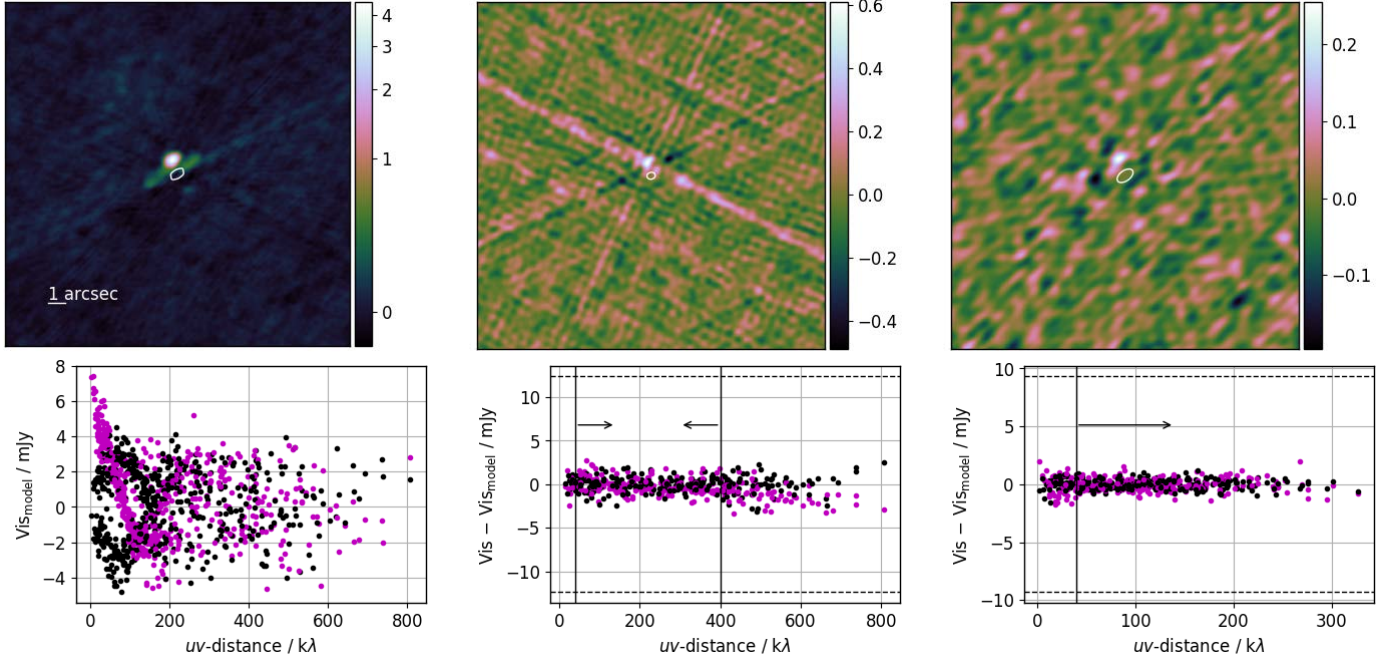

**Figure A40.** Model and residual plots for PCCS1 030 G134.59-50.34; see caption for Fig. A39 for more detail. The model has been self-calibrated using the common  $uv$ -range indicated by the solid vertical black lines, and the residual plots produced using this  $uv$ -range.

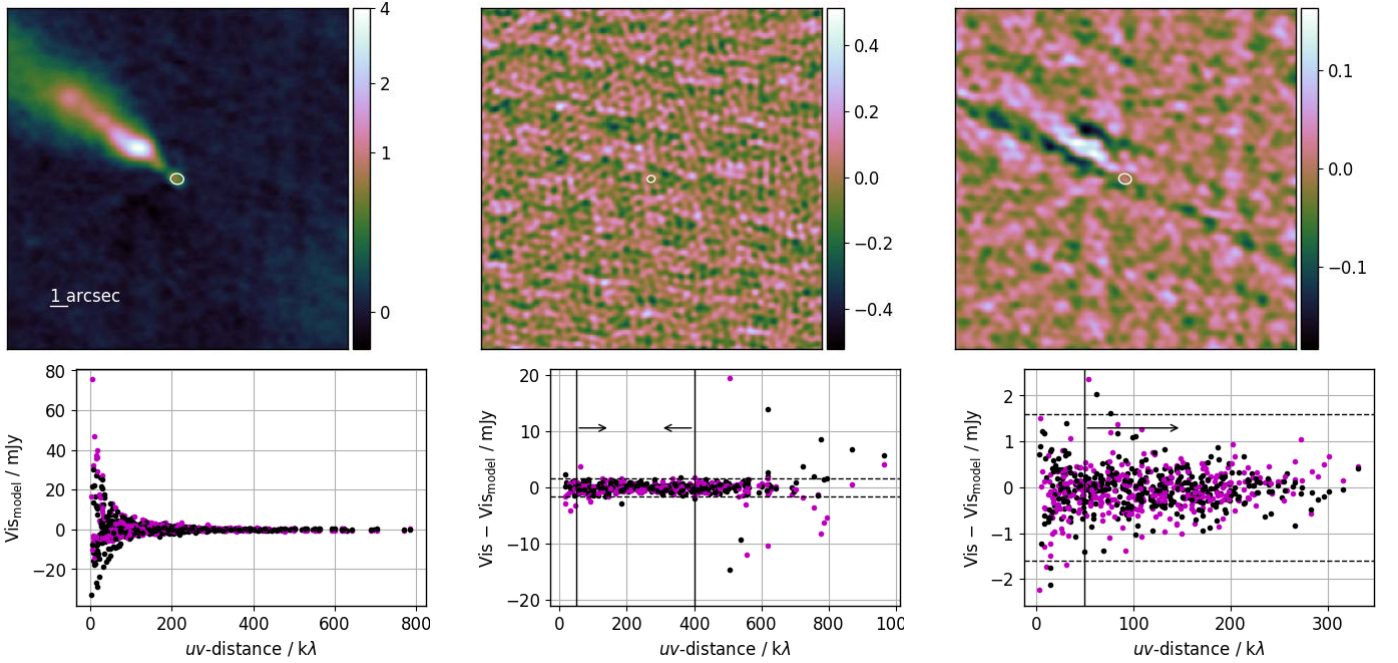

**Figure A41.** Model and residual plots for PCCS1 030 G140.23-16.73; see caption for Fig. A39 for more detail. The model has been self-calibrated using the common  $uv$ -range indicated by the solid vertical black lines, and the residual plots produced using this  $uv$ -range.

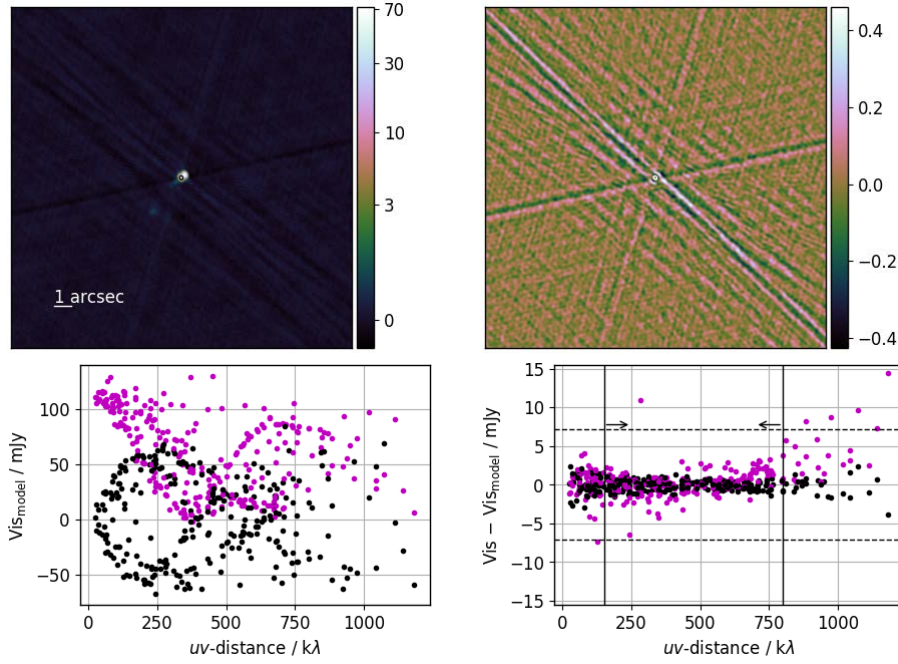

**Figure A42.** Model and residual plots for PCCS1 030 G182.17+34.17; see caption for Fig. A39 for more detail. In this case there is only one observing epoch. The model has been self-calibrated using the  $uv$ -range indicated by the solid vertical black lines, and the residual plots produced using this  $uv$ -ranges.

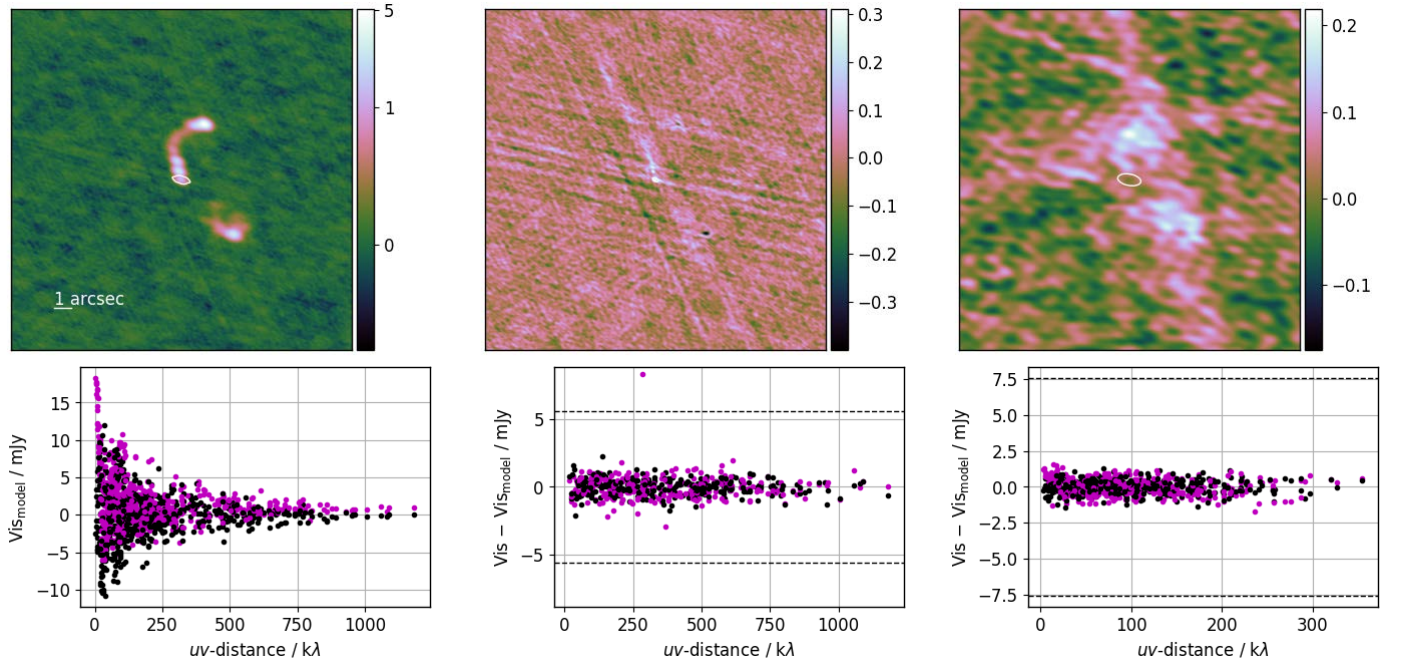

**Figure A43.** Model and residual plots for PCCS1 030 G133.79+42.34; see caption for Fig. A39 for more detail.

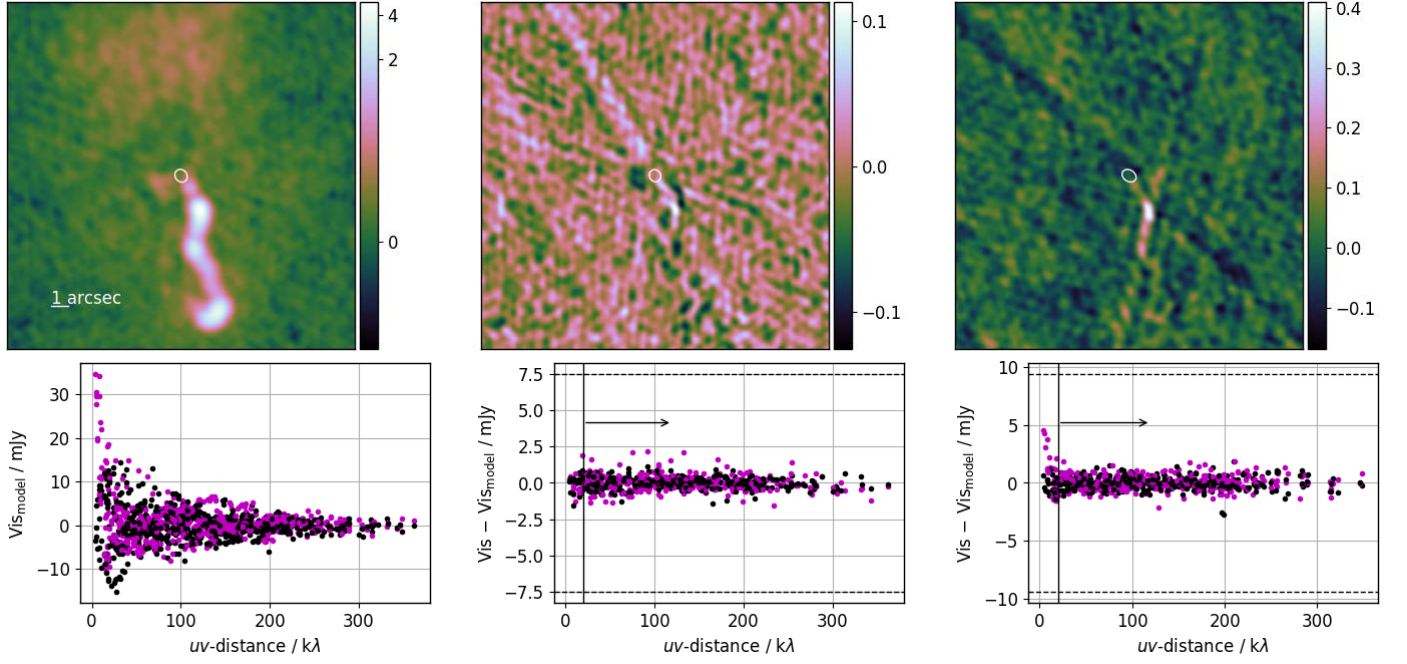

**Figure A44.** Model and residual plots for PCCS1 030 G145.65+64.96; see caption for Fig. A39 for more detail. The model has been self-calibrated using the common  $uv$ -limit indicated by the solid vertical black lines, and the residual plots produced using this  $uv$ -limit.

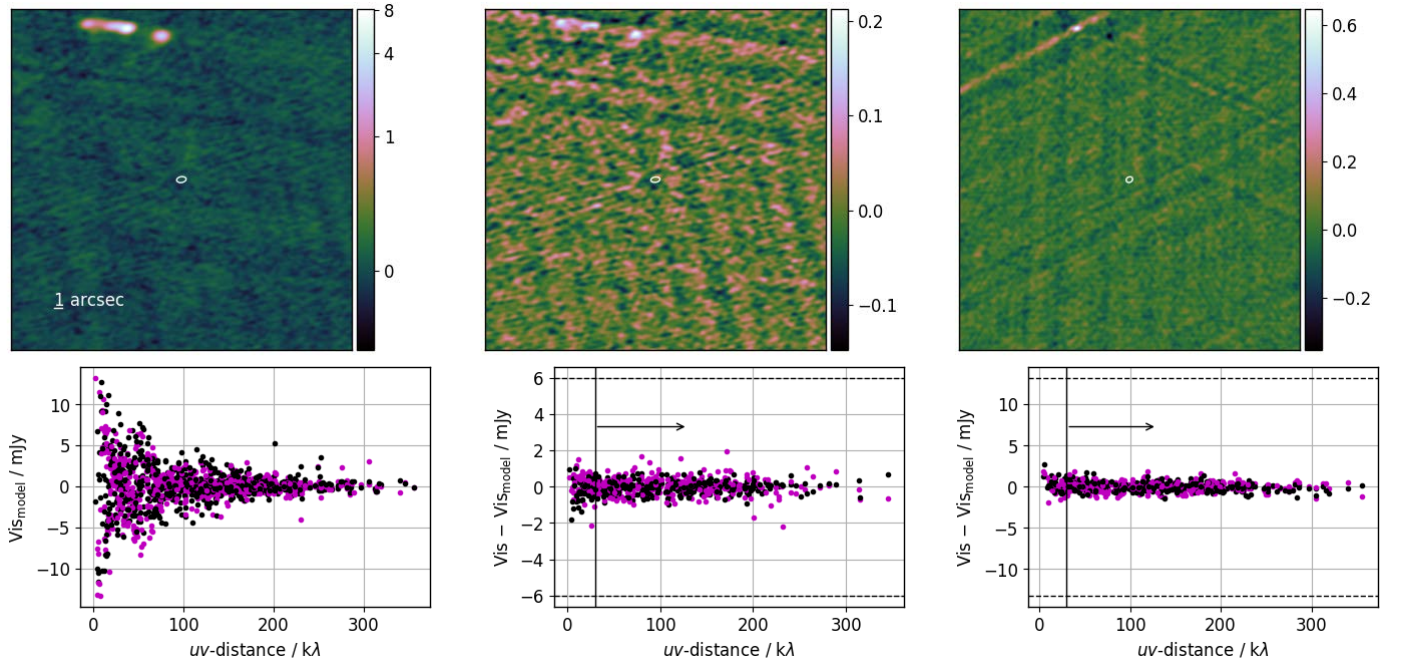

**Figure A45.** Model and residual plots for PCCS1 030 G073.40+41.88; see caption for Fig. A39 for more detail. The model has been self-calibrated using the common  $uv$ -limit indicated by the solid vertical black lines, and the residual plots produced using this  $uv$ -limit. The source visible is an unrelated AGN, [RPG99] 1636+473 B. The core appears to have brightened and the hot-spots dimmed between the two observations. We also self-calibrated each observation individually; the fitted core flux density and spectral index changed by much less than the calibration errors compared to the jointly self-calibrated results.

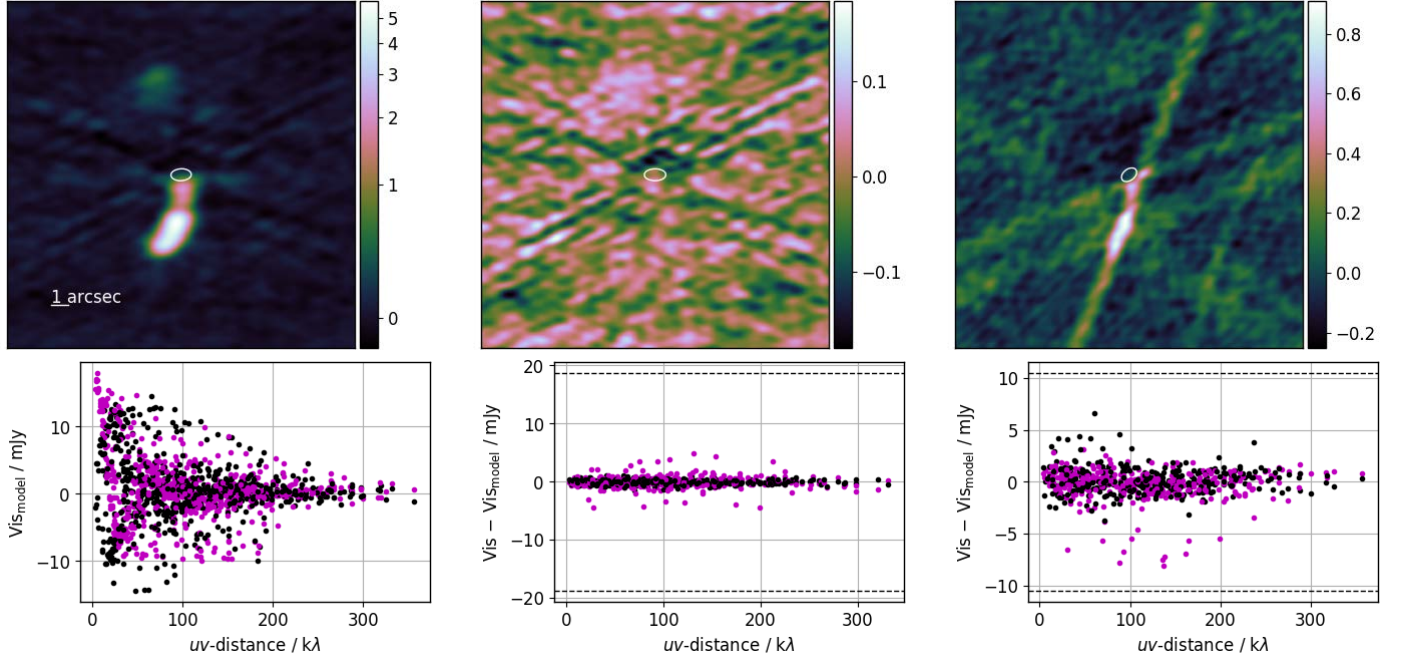

**Figure A46.** Model and residual plots for PCCS1 030 G100.68+36.62; see caption for Fig. A39 for more detail.

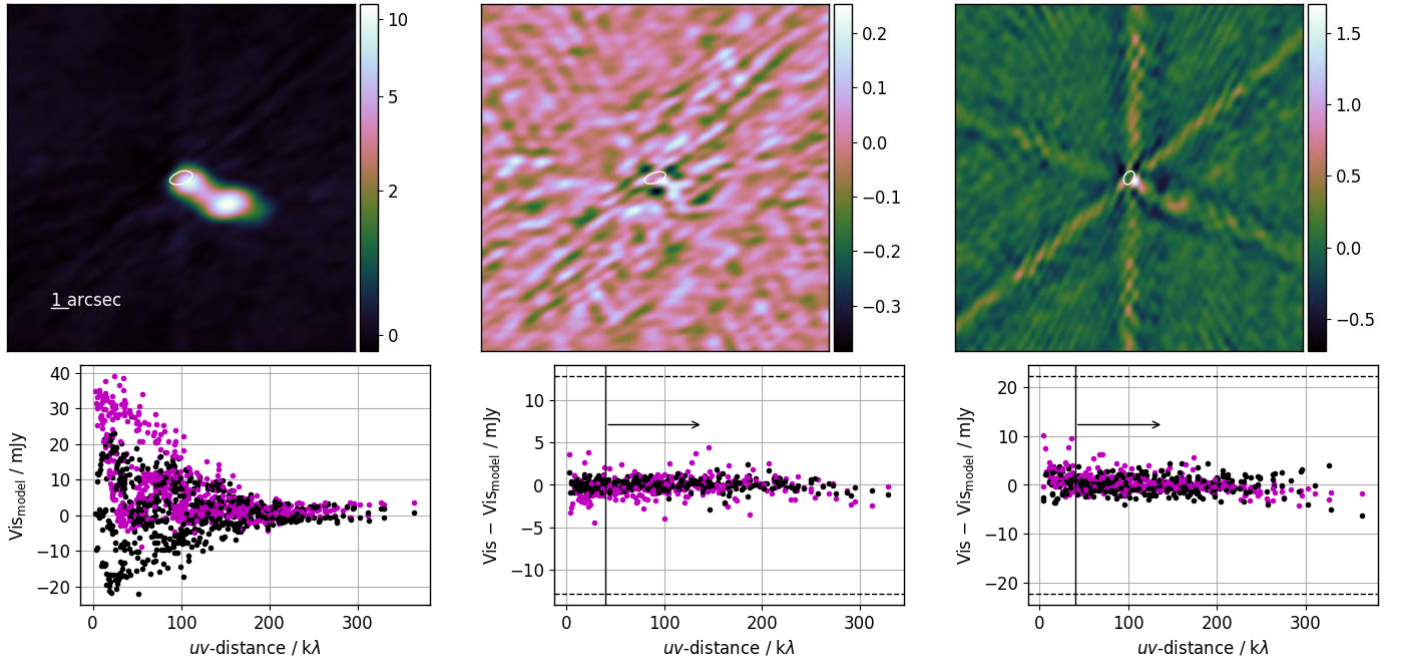

**Figure A47.** Model and residual plots for PCCS1 030 G100.13+29.16; see caption for Fig. A39 for more detail. The model has been self-calibrated using the common  $uv$ -limit indicated by the solid vertical black lines, and the residual plots produced using this  $uv$ -limit.

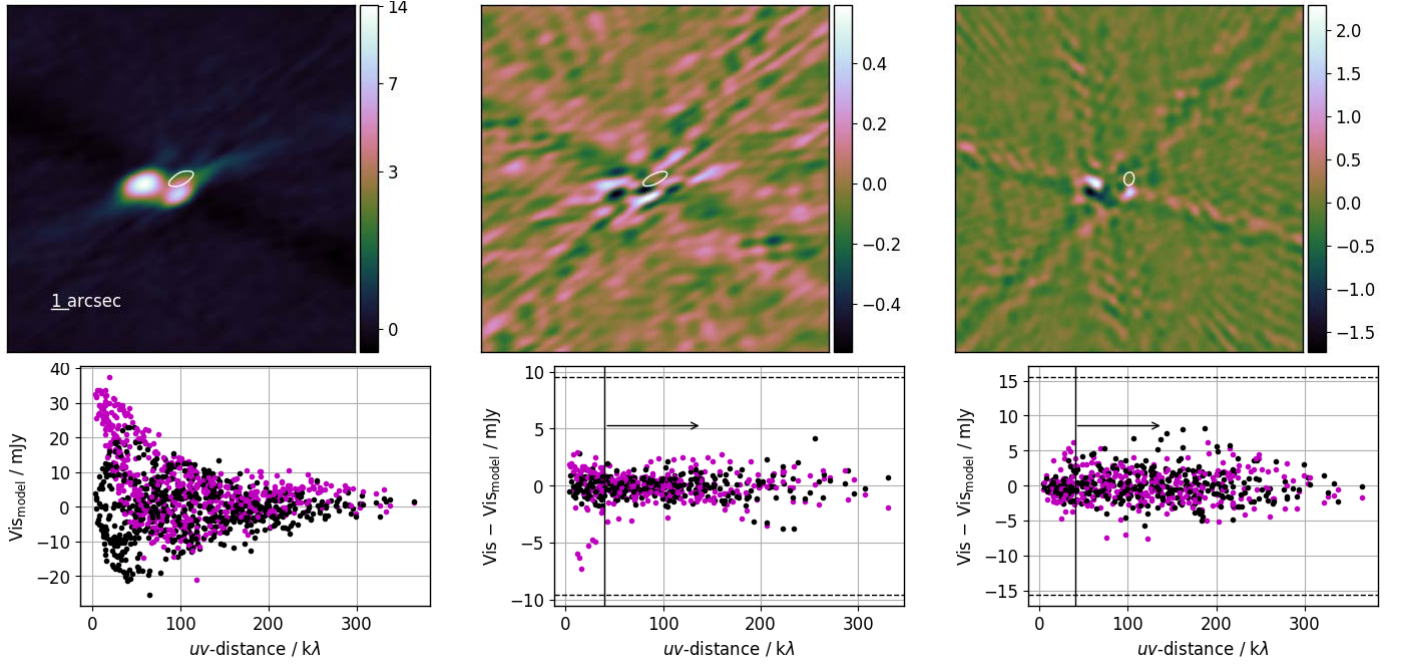

**Figure A48.** Model and residual plots for PCCS1 030 G085.73+26.11; see caption for Fig. A39 for more detail. The model has been self-calibrated using the common  $uv$ -limit indicated by the solid vertical black lines, and the residual plots produced using this  $uv$ -limit.

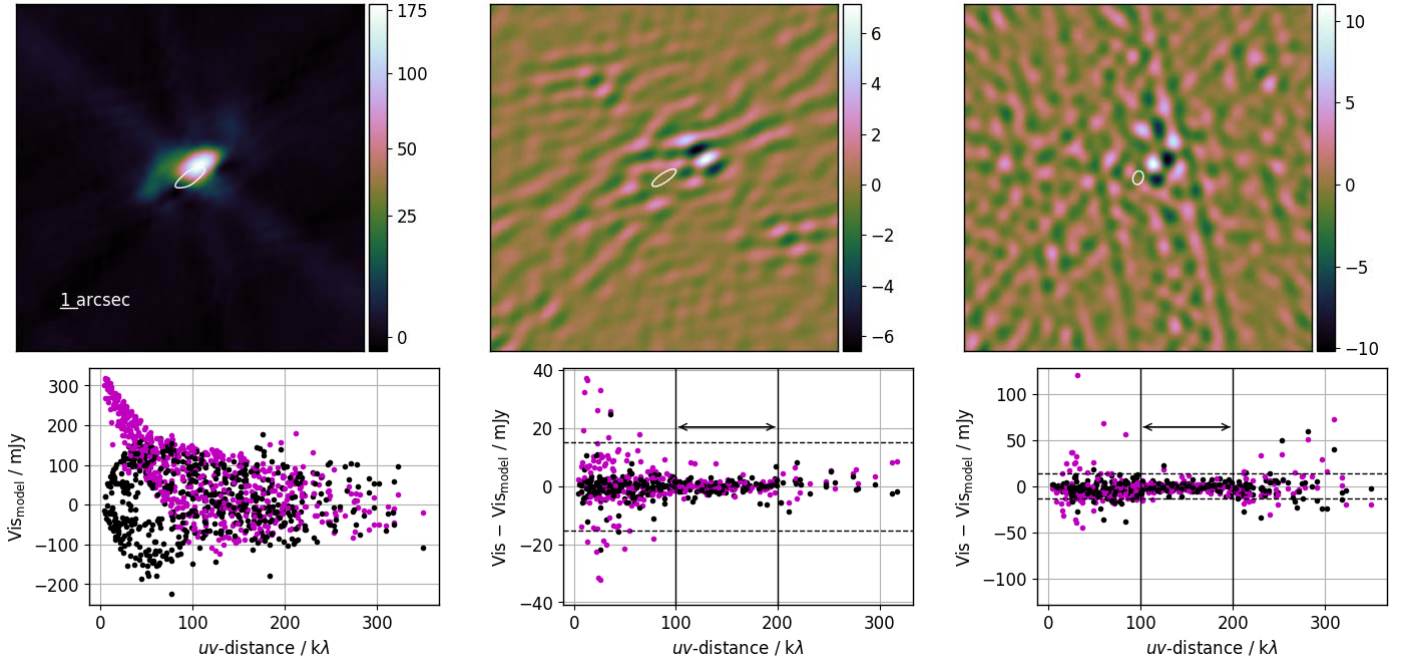

**Figure A49.** Model and residual plots for PCCS1 030 G077.23+23.50; see caption for Fig. A39 for more detail. The extended structure around this source varied significantly between the two observations, as also seen in Koyama et al. (2013) (see text for more detail). The black vertical lines indicate the  $uv$ -range over which we found the best agreement between the observations, and we used this range for calibration and to produce the residual plots. When self-calibrating these observations individually, the amplitude solution for the source changed by  $\approx 2\%$  and the spectral index by  $\approx 0.1$  compared to the combined result; we therefore take the individually calibrated results as our fiducial values and add an extra 2% and 0.1 uncertainty to the overall calibration errors in central flux density and spectral index, respectively.

**A3 Extended sources**

In two cases only, PCCS1 030 G157.08-42.72 and PCCS1 030 G147.84-44.04, the self-calibration method failed because the diffuse emission did not cleanly separate from the compact core. In these cases, we followed a slightly different method. We first self-calibrated each individual observation (without subtracting a point-source component). Then, we verified that the difference between the self-calibrated observations, in the common  $uv$ -range, was consistent with a point source, i.e. the variation was dominated by the variation of a compact core. We then added the point-source difference to one of the observations so they could be imaged together, and self-calibrated the combined observation in the common  $uv$ -range, iteratively improving the estimate of the point-source difference. Finally, we used the model to estimate the total combined flux density (including the diffuse component) at the smallest common  $uv$ -distance, for each observation. The flux density and spectral index estimates therefore differ from the other sources in that they include the extended component; but the variation between observations is dominated by the compact core as in the rest of the sample.

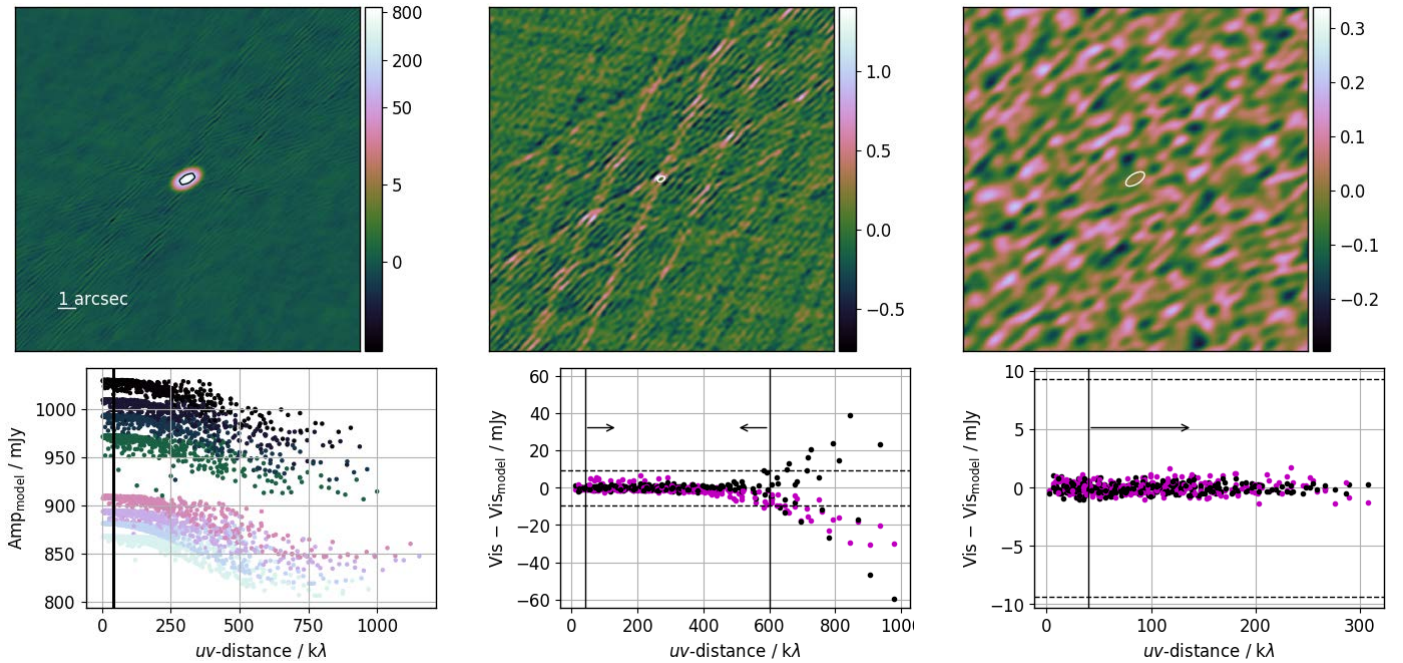

**Figure A50.** Model and residual plots for PCCS1 030 G147.84-44.04. The model plots (left-hand column) show the combined total model, i.e. observation 1 combined with observation 2 + point source difference. In the  $uv$ -plane model plot, the visibilities have been averaged over all time and into eight frequency bands; the points are colour-coded by frequency (frequency increasing from dark to light colours) and for clarity only the amplitude is shown. The residual plots (centre and right-hand columns) show fully-subtracted maps and visibility real and imaginary components for each observation, i.e. observation 1 self-calibrated data – combined total model and observation 2 self-calibrated data – combined total model – point source difference. As in Fig. A1, the colour-scale for the maps is in mJy/beam; the angular scale is indicated with the horizontal line on the left-hand map and the 50% contour of the synthesised beam is shown at the position of the subtracted point source on each map. The field of view is the same in the three maps. The residual maps have not been cleaned. In the residual  $uv$ -plane plots, the visibility data have been averaged over frequency (28 – 40 GHz) and time to leave one point per baseline; magenta and black points are real and imaginary components respectively. The horizontal black dashed lines on the residual  $uv$ -plane plots indicate 1% of the ‘total’ flux density at the central frequency at each epoch, as measured at the shortest common  $uv$ -distance indicated by the thick vertical black line on the model  $uv$ -plane plot. The model has been self-calibrated using the common  $uv$ -range indicated by the solid vertical black lines on the residual plots, and the residual maps produced using this  $uv$ -range.

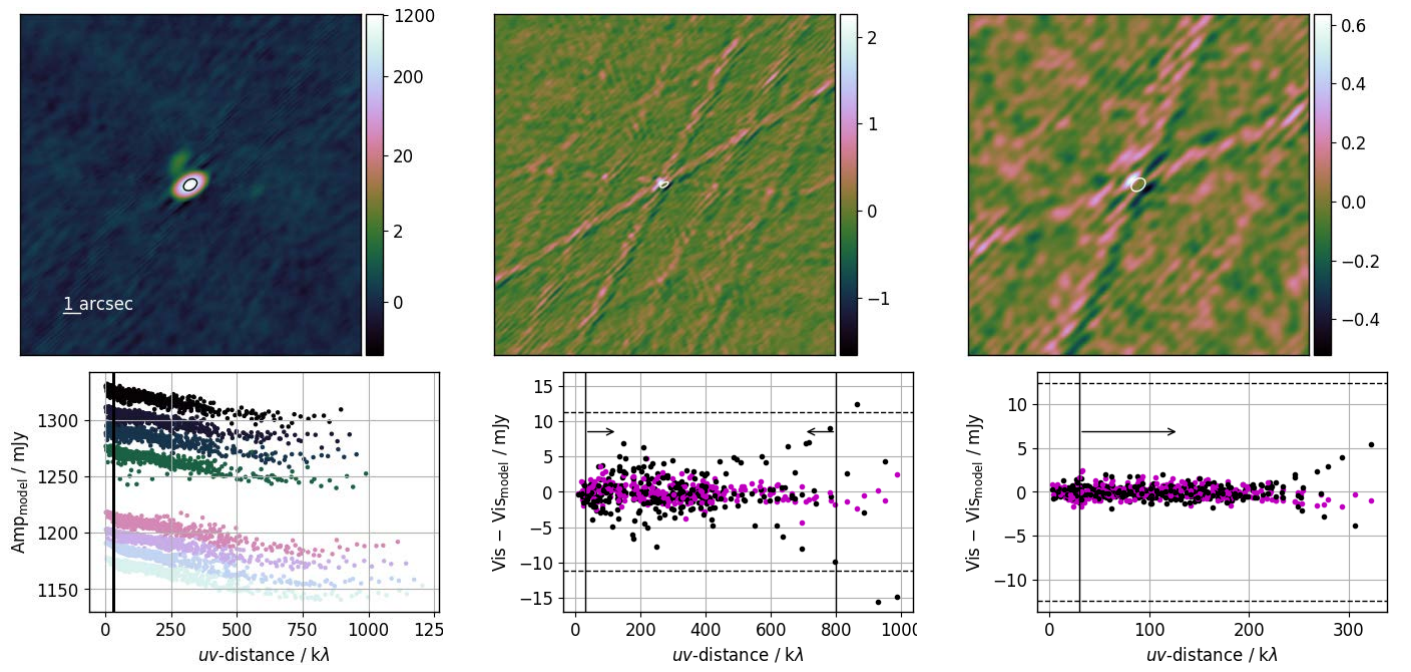

**Figure A51.** Model and residual plots for PCCS1 030 G157.08-42.72; see caption for Fig. A50 for more detail.

## References

- Koyama S., et al., 2013, PASJ, 65, 29  
Papageorgiou A., et al., 2006, MNRAS, 373, 449
